# Supplementary material for: Spontaneous phase coordination and fluid pumping in model ciliary carpets
Source: arXiv:2208.10811 source file (2022-09-21)
Supplement: Supplementary file 1 [file Supplemental_Information.pdf]

Supplemental Materials for

# Spontaneous phase coordination and fluid pumping in model ciliary carpets

Anup V Kanale[1], Feng Ling[1], Hanliang Guo[1,2,3], Sebastian Fürthauer[4,5], Eva Kanso[1*]

[1]Aerospace and Mechanical Engineering, University of Southern California, Los Angeles, CA 90089, USA.
[2]Department of Mathematics, University of Michigan, Ann Arbor, MI 48109, USA.
[3]Department of Mathematics and Computer Science, Ohio Wesleyan University, Delaware, OH 43015, USA.
[4]Center for Computational Biology, Flatiron Institute, New York, NY 10010, USA.
[5]Institude for Applied Physics, TU Wien, 1050 Wien, Austria.

## S.1 Stokes Flow Solution

Consider the cilia to be submerged in a viscous fluid domain consisting of an infinite three-dimensional (3D) half space, bounded by a flat substrate at $z = 0$. Our goal is to solve the incompressible Stokes equations

$$\eta \Delta \mathbf{u} = -\nabla p, \qquad \nabla \cdot \mathbf{u} = 0, \tag{1}$$

for two ciliary models: (1) we consider each cilium as a force monopole $\mathbf{F}$, and the ciliary carpet as a 2D lattice of force monopoles; (2) we take the limit of infinitely-many cilia and we consider the collection of all cilia to form a ciliary plane that is exerting a force density $\mathbf{f}(\mathbf{x})$ on the fluid.

### S.1.1 Blake-Oseen Solution in the 3D Half-Space

**Fluid velocity induced by a force monopole in the 3D half-space.** Consider a point force $\mathbf{F}$ acting at a point $\mathbf{x}_0 = (x_0, y_0, z_0)$, at a distance $z_0 = h$ above a no-slip wall. The velocity induced at a point $\mathbf{x} = (x, y, z)$ in the 3D half-space is given by

$$\mathbf{u}(\mathbf{x}) = \mathbf{B}(\mathbf{x}, \mathbf{x}_0) \cdot \mathbf{F}, \tag{2}$$

where $\mathbf{B}(\mathbf{x}, \mathbf{x}_0)$ is the Blake-Oseen tensor. Starting from the Green-Oseen solution associated with the point force $\mathbf{F}(\mathbf{x}_0)$ in the unbounded 3D space, where the velocity field $\mathbf{v}(\mathbf{x}) = \mathbf{S}(\mathbf{x}, \mathbf{x}_0) \cdot \mathbf{F}$ is obtained from the Green-Oseen tensor, Blake [1] constructed an image system to satisfy the no-slip condition at the wall, by placing a combination of higher order singularities at a reflected point about the z-axis, $\mathbf{x}_0^I = (x_0, y_0, -z_0)$,

$$\mathbf{B}(\mathbf{x}, \mathbf{x}_0) = \mathbf{S}(\mathbf{x}, \mathbf{x}_0) - \mathbf{S}(\mathbf{x}, \mathbf{x}_0^I) + 2h^2 \mathbf{S}^D(\mathbf{x}, \mathbf{x}_0^I) - 2h \mathbf{S}^{SD}(\mathbf{x}, \mathbf{x}_0^I). \tag{3}$$

Here, the Green-Oseen tensor (also known as the Stokeslet solution or solution) is given by

$$\mathbf{S}(\mathbf{x}, \mathbf{x}_0) = \frac{1}{8\pi\eta|\mathbf{x} - \mathbf{x}_0|}\left(\mathbf{I} + \frac{(\mathbf{x} - \mathbf{x}_0) \otimes (\mathbf{x} - \mathbf{x}_0)}{|\mathbf{x} - \mathbf{x}_0|^2}\right), \tag{4}$$

*kanso@usc.edu

and $\mathbf{S}^D$ and $\mathbf{S}^{SD}$ are the modified source and Stokes doublets, respectively,

$$\begin{aligned}\mathbf{S}^D(\mathbf{x},\mathbf{x}_0) &= \frac{1}{8\pi\eta}\mathbf{P}\cdot\boldsymbol{\nabla}\frac{\mathbf{x}-\mathbf{x}_0}{|\mathbf{x}-\mathbf{x}_0|},\\ \mathbf{S}^{SD}(\mathbf{x},\mathbf{x}_0) &= \mathbf{P}\cdot\boldsymbol{\nabla}\left(\mathbf{S}(\mathbf{x},\mathbf{x}_0)\cdot\mathbf{e}_z\right),\end{aligned} \tag{5}$$

where $\mathbf{P}$ is a $3\times 3$ matrix with diagonal elements $[1,1,-1]$ and all the non-diagonal elements equal to zero. We refer the reader to the original work [1] for a detailed derivation, and [2] for a convenient, physically intuitive reformulation.

**Fluid velocity induced by a discrete lattice of forces** Consider a large number of force monopoles placed at discrete locations, say $\mathbf{x}_i$, $i = 1,\dots N$ on a 2D square lattice, of base distance $d$ between neighboring vertices and fundamental domain of size $L\times L$. Here, $N$ is the total number of force monopoles in the fundamental domain. We can define the 'density' of cilia $\rho_c = N/L^2$ as the total number of force monopoles per unit area.

Our goal is to evaluate the fluid velocity $\mathbf{u}$ at the location of the force monopole $i$ in the fundamental domain (red square in Fig. S.2B) induced by all other force monopoles ($j\neq i$) in the fundamental and periodic image domains (red and grey squares in Fig. S.2B). Theoretically, one has a doubly-infinite image system that tiles the entire 2D plane, and to compute the fluid velocity, one needs to take a doubly-infinite sum of the right-hand size of (2) over all force monopoles [3, 4]. This doubly-infinite sum is conditionally-convergent because of the quadratic decay of the Blake-Oseen tensor $\mathbf{B}$ in (2). Here, we relax the requirement of an infinite lattice (no ciliated tissue extends to infinity), and we consider hydrodynamic interactions between cilia in the fundamental domain and a finite number of image domains.

### S.1.2 Fluid Velocity in Continuum Force Density Layer

Our goal is to solve the incompressible Stokes equations (1) subject to the force density that the cilia exert on the fluid

$$\mathbf{f}(\mathbf{x}) = \lim_{N\to\infty}\sum_{j=1}^{N}\mathbf{F}_j\delta(\mathbf{x}-\mathbf{x}_j). \tag{6}$$

where $\delta(\mathbf{x}-\mathbf{x}_j)$ has units of inverse area. Here, all forces are exerted within the thin 2d layer at a distance $h$ above the surface on which cilia are embedded (see Fig. 1B of main text). To solve for the fluid velocity field $\mathbf{u}$ that the force density $\mathbf{f}$ induces, we adapt the method in [5–7] concerning the flows generated by a 2d force layer in an infinite fluid to the geometry of our ciliary system, as discussed next.

**Setting up the Stokes equations and boundary conditions.** Given that the force density $\mathbf{f}(\mathbf{x})$ in (6) is confined to a layer at $z = h$, we partition space into two domains above and below the layer, which we denote by the '+' and '−' superscripts respectively. Rewriting the incompressible Stokes equations in each domain gives

$$\begin{aligned}&\eta\nabla^2\mathbf{u}^+ - \nabla p^+ = 0, \qquad \nabla\cdot\mathbf{u}^+ = 0, \qquad z\in(h,\infty),\\ &\eta\nabla^2\mathbf{u}^- - \nabla p^- = 0, \qquad \nabla\cdot\mathbf{u}^- = 0, \qquad z\in[0,h).\end{aligned} \tag{7}$$

Due to the ciliary force layer at $z = h$, the stress field $\boldsymbol{\sigma} = -p\mathbf{I} + \eta\left(\nabla\mathbf{u} + (\nabla\mathbf{u})^T\right)$ experiences a jump

$$[\![\boldsymbol{\sigma}\cdot\mathbf{e}_z]\!]_{z=h} = \boldsymbol{\sigma}\cdot\mathbf{e}_z|_{z=h^+} - \boldsymbol{\sigma}\cdot\mathbf{e}_z|_{z=h^-} = \mathbf{f}(\mathbf{x}). \tag{8}$$

In addition, we impose a no-slip condition at the substrate

$$\mathbf{u}^{-}(x, y, z=0) = 0, \tag{9}$$

and velocity continuity at the ciliary layer

$$\mathbf{u}^{+}(x, y, z^{+} \to h) = \mathbf{u}^{-}(x, y, z^{-} \to h). \tag{10}$$

We also require the pressure and velocity to be bounded in the far field

$$\lim_{z\to\infty} p^{+} = 0, \qquad \lim_{z\to\infty} \mathbf{u}^{+} = \text{constant}. \tag{11}$$

This choice captures the physics of vanishing wall shear stress at $z \to \infty$, such as one would for instance expect at a water air interface far above the ciliary layer.

**Analytical solution of fluid velocity.** We decompose the fluid velocity field $\mathbf{u}(x, y, z)$ into a horizontal component $\mathbf{v}(x, y, z) = (\mathbf{u}\cdot\mathbf{e}_x)\mathbf{e}_x + (\mathbf{u}\cdot\mathbf{e}_y)\mathbf{e}_y$ and a vertical component $w(x, y, z) = \mathbf{u}\cdot\mathbf{e}_z$. To solve (8)–(11), we take the Fourier transform with respect to the in-plane coordinates $\mathbf{x} = (x, y)$ [6, 7]. Using $\mathbf{k} = (k_x, k_y)$ for the in-plane wavenumber coordinates, the momentum equations in (7) become

$$\begin{aligned} i\mathbf{k}\cdot\hat{\mathbf{v}}^{\pm} + \partial_z \hat{w}^{\pm} &= 0, \\ \eta(\partial_{zz} - k^2)\hat{\mathbf{v}}^{\pm} - i\mathbf{k}\hat{p}^{\pm} &= 0, \\ \eta(\partial_{zz} - k^2)\hat{w}^{\pm} - \partial_z \hat{p}^{\pm} &= 0, \end{aligned} \tag{12}$$

where hatted quantities denote the in-plane Fourier transforms of their physical space equivalents, and $k = \|\mathbf{k}\|$ is the magnitude of the 2D wave number vector. Since the fluid is incompressible, the pressure obeys a Poisson equation. In Fourier space, this is given by

$$(\partial_{zz} - k^2)\hat{p}^{\pm} = 0, \tag{13}$$

which is solved by

$$\hat{p}^{\pm} = A^{\pm} e^{-k(z-h)} + B^{\pm} e^{k(z-h)}, \tag{14}$$

where $A^{\pm} = A^{\pm}(\mathbf{k})$ and $B^{\pm} = B^{\pm}(\mathbf{k})$ are constants of integration to be determined from the boundary conditions. Substituting (14) into (12) and solving for $\mathbf{v}^{\pm}$ and $w^{\pm}$ gives

$$\begin{aligned} \hat{\mathbf{v}}^{\pm} &= \left(\mathbf{O}^{\pm} - \frac{i\mathbf{k}A^{\pm}}{2\eta k}(z-h)\right) e^{-k(z-h)} + \left(\mathbf{Q}^{\pm} + \frac{i\mathbf{k}B^{\pm}}{2\eta k}(z-h)\right) e^{k(z-h)}, \\ \hat{w}^{\pm} &= \left(C^{\pm} + \frac{A^{\pm}}{2\eta}(z-h)\right) e^{-k(z-h)} + \left(D^{\pm} + \frac{B^{\pm}}{2\eta}(z-h)\right) e^{k(z-h)}. \end{aligned} \tag{15}$$

Using the boundary condition (8)–(11) we finally arrive at

$$\hat{\mathbf{v}} = \hat{\mathbf{K}}\cdot\hat{\mathbf{f}}, \tag{16}$$

with $\hat{\mathbf{K}}(k_x, k_y)$ encodes the Stokes kernel associated with the infinite force density layer at $z = h$,

$$\hat{\mathbf{K}} = \begin{cases} \dfrac{1}{4\eta k^3}\left[\, 2k^2(1 - e^{-2kh})\mathbf{I} + ((1 + 2kh - 2k^2h^2)\, e^{-2kh} - 1)\mathbf{k}\otimes\mathbf{k} \,\right], & \mathbf{k} \neq 0, \\ \dfrac{h}{\eta}\mathbf{I}, & \mathbf{k} = 0. \end{cases} \tag{17}$$

**Solving for the unknown coefficients.** To solve for the unknown coefficients $A^{\pm}$, $B^{\pm}$, $C^{\pm}$, $D^{\pm}$, $\mathbf{O}^{\pm}$, $\mathbf{Q}^{\pm}$ in (14) and (15), we first apply the boundedness condition of (11) as $z \to \infty$ to eliminate the exponentially growing terms in (14) and (15). Substituting the resulting expressions into (12) and matching coefficients leads to

$$i\mathbf{k} \cdot \mathbf{O}^{+} - kC^{+} + \frac{A^{+}}{2\eta} = 0. \tag{18}$$

Similarly, substituting expressions for $\hat{p}^{-}$, $\hat{\mathbf{v}}^{-}$ and $w^{-}$ into equation (12) and matching coefficients leads to

$$i\mathbf{k} \cdot \mathbf{O}^{-} - kC^{-} + \frac{A^{-}}{2\eta} = 0, \qquad i\mathbf{k} \cdot \mathbf{Q}^{-} + kD^{-} + \frac{B^{-}}{2\eta} = 0. \tag{19}$$

Next, we enforce the no-slip condition (10) at $z = 0$ to obtain

$$\begin{gathered} \left(\mathbf{O}^{-} + \frac{ih\mathbf{k}A^{-}}{2\eta k}\right) e^{kh} + \left(\mathbf{Q}^{-} - \frac{ih\mathbf{k}B^{-}}{2\eta k}\right) e^{-kh} = 0, \\ \left(C^{-} - \frac{hA^{-}}{2\eta}\right) e^{kh} + \left(D^{-} - \frac{hB^{-}}{2\eta}\right) e^{-kh} = 0. \end{gathered} \tag{20}$$

By continuity of velocity at $z = h$, we get

$$C^{+} = C^{-} + D^{-}, \qquad \mathbf{O}^{+} = \mathbf{O}^{-} + \mathbf{Q}^{-} \tag{21}$$

Finally, we turn to the jump condition (8) at the ciliary layer. In component form, $\boldsymbol{\sigma} \cdot \mathbf{e}_z$ can be expressed as $\boldsymbol{\sigma} \cdot \mathbf{e}_z = \left(\eta(\partial_z u + \partial_x w), \eta(\partial_z v + \partial_y w), -p + 2\eta \partial_z w\right)$, which can be rewritten in Fourier space as $\hat{\boldsymbol{\sigma}} \cdot \mathbf{e}_z = \left(\eta(\partial_z \hat{\mathbf{v}} + i\mathbf{k}\hat{w}), -\hat{p} + 2\eta \partial_z \hat{w}\right)$. Evaluating $\hat{\boldsymbol{\sigma}} \cdot \mathbf{e}_z$ at $z = h^{+}$ and $z = h^{-}$ and matching the jump in (8) gives

$$\eta k(\mathbf{O}^{+} - \mathbf{O}^{-} + \mathbf{Q}^{-}) + \frac{i\mathbf{k}}{2k}(A^{+} - A^{-} + B^{-}) = \hat{\mathbf{f}}, \qquad 2\eta k(C^{+} - C^{-} + D^{-}) = 0. \tag{22}$$

where $\hat{\mathbf{f}} = (\hat{f}_x, \hat{f}_y)$ and the vertical component of $\mathbf{f}$ is identically zero by construction. Equations (18)-(22) form a closed system of algebraic equations that we solve analytically to obtain the coefficients $A^{\pm}$, $B^{\pm}$, $C^{\pm}$, $D^{\pm}$, $\mathbf{O}^{\pm}$, $\mathbf{Q}^{\pm}$.

### S.1.3 Comparing Flow Fields in Discrete and Continuum Models

We compare the flow-fields induced by ciliary carpets in the two models: (1) the particle model that uses direct summation of the Blake tensor with interaction stencil (§ S.1.1), and (2) the continuum model that uses the expression $\hat{\mathbf{v}}(\mathbf{k}) = \hat{\mathbf{K}}(\mathbf{k}) \cdot \hat{\mathbf{f}}(\mathbf{k})$ (§ S.1.2).

In the discrete theory, wavenumbers lie in the range $[2\pi/L, \pi/d]$, where $2\pi/L$ is the wavenumber associated with the periodic square domain. In the continuum theory, periodicity is implicit by virtue of expressing the model in Fourier space. In all figures, we use the wavenumber resolution $\Delta k = 2\pi/L$. The maximum wavenumber is $k_{max} = 2\pi/\Delta x$, where $\Delta x$ is the grid resolution in the physical space. We evaluate $\hat{\mathbf{v}}(\mathbf{k})$ at each wavenumber $\mathbf{k}$ and we invert it numerically to get the velocity field $\mathbf{u}(x, y, z)$ in physical space.

Fig. S.3 shows the flow field generated by a single force monopole (cilium) placed above a no-slip wall; Fig. S.3A shows the in-plane flowfield, Fig. S.3B shows the flowfields in a plane perpendicular to the plane of the cilium, and Fig. S.3C shows the absolute value of the difference in the $x$-component of the velocity vector $\mathbf{u}(x, y, z = h)$ between the discrete and continuum models along the two lines $x = 0$ and $y = 0$. The agreement away from the force singularities is remarkable. Figs. S.4 and S.5 compares the flow fields generated by a $5 \times 5$ lattice of cilia in the two configurations of interest – isotropic (Fig. S.4) and fully synchronized (Fig. S.5) states – again showing remarkable agreement between the two methods for computing the fluid velocity field.

# S.2 Discrete Rotor Model

To investigate the emergent coodination in tens of thousands of hydrodynamically-coupled cilia, we use a discrete model where each cilium is represented as a nonlinear phase oscillator. Here, we first provide an interpretation of the phase oscillator model in light of the distinctive features of biological cilia beating patterns. Then, to fix ideas on the role of metachronal coordination in fluid pumping, we present a case study in a 1D array of ten cilia. Lastly, we discuss the equations of motion and algorithm we use to compute emergent coordination in tens of thousands of hydrodynamically-interacting cilia.

## S.2.1 Modeling Individual Cilia as Nonlinear Phase Oscillators

**Biological cilia beating patterns.** To overcome the instantaneity of Stokes' flow and pump fluid at the micron scale where viscosity is dominant [8], individual cilia tend to adopt an asymmetric beating cycle that consists of an effective and a recovery stroke; see Fig. S.1A. Crucially, the exact form of these strokes can be regulated differently depending on the species or even on different parts of a single organism as their fluid pumping functions differs; *e.g.,* oral-groove cilia for feeding can exhibit intrinsically different beating characteristics than body cilia primarily responsible for locomotion [9]. Another important characteristic of natural cilia beating patterns is that while some cilia confine their motion to a two-dimensional plane, many cilia and eukaryotic flagella adopt intrinsically three-dimensional, cone-like, beating trajectories [10] (see Fig. S.1D). The amount and type of asymmetry and geometry of cilia beats play important role in cilia synchronization [11,12]. We next show that these key features of the ciliary beating patterns – stroke asymmetry and 3D ellipticity – can be captured in the context of reduced-order phase oscillator models.

**Rotor model.** To study synchronization of beating cilia, reduced-order models of cilia beating patterns have been proposed in the form of nonlinear phase oscillators that capture the cyclic motion of the beating cilium. These models are particularly attractive for studying large arrays of hydrodynamically coupled cilia in an efficient manner. Rotor and rower models have been proposed [13–18]. In both models, the cilium is represented by a force monopole. In the rotor model, the force monopole traces a closed trajectory, while in the rower model, the force monopole oscillates along a line segment [19–21].

To capture the two main features of actual cilia beating patterns – stroke asymmetry and 3D ellipticity – the geometric features of the rotor model can be manipulated. For example, a trajectory that is titled relative to a bounding plane accounts for stroke asymmetry and can lead to fluid pumping [22, 23]. A force monopole tracing an elliptic trajectory, without tilt, accounts for 3D geometric ellipticity.

**Interpretation of active force in our rotor model in light of cilia beating patterns.** Our goal is to study the synchronization of rotors, where each rotor consists of a bead moving along a horizontal circle placed above and parallel to a no-slip wall. Each rotor is characterized by its angle $\theta$ along the circular trajectory and is driven by a tangential force $F(\theta)$, similar to models introduced in [16–18]. Generically, the force $F(\theta)$ can be written as an infinite sum

$$F(\theta) = F_o \left( 1 + \sum_{m=1}^{\infty} \alpha_m \cos m\theta + \beta_m \sin m\theta \right), \tag{23}$$

where $\alpha_m$ and $\beta_m$ are coefficients of the Fourier series expansion of $F$ in terms of $\theta$. In the following, we demonstrate that the *first harmonic* forcing ($m = 1$) captures the asymmetry of the beating pattern without inducing a net flux, and the *second harmonic* forcing ($m = 2$) serves to isolate the effect of non-planar ellipticity of cilia beating.

We prove these statements using a simple approach: starting from rotors that are known to represent stroke asymmetry and 3D ellipticity of generic cilia beating, we show that we can produce similar far-field fluid velocity using the circular rotor model by proper choice of force harmonics. To represent beat asymmetry, we consider a circular rotor tilted with respect to the bounding wall. To isolate the effect of non-planar beating, we consider a rotor consisting of an ellipitcal orbit parallel to the wall; see Fig. S.1A,B. In both cases, the rotor moves under a tangential force of constant magnitude. We use (2) to calculate the instantaneous flow field $\mathbf{u}(\mathbf{x})$ induced at a regular 3D grid suffficently far away from the rotor, and we use these values in a nonlinear least squares fit to obtain the magnitude of a tangential force $F(\theta)$ applied by a *circular* rotor; see Fig. S.1C,F. That is, we solve for optimal $F(\theta)$ the minimizes the error in the far-field fluid velocity created by the titled and elliptic rotors and that created by a non-tilted circular rotor. The optimization results show that, to leading order, the tilt representing beat asymmetry can be captured by a equivalent *circular* rotor with a phase-dependent forcing that oscillates exactly *once* sinusoidally along one full rotation cycle, i.e., a first force harmonic (Fig. S.1C), while an elliptical beat trajectory can be captured by a phase-dependent forcing that oscillates *twice* sinusoidally along one full rotation cycle, i.e., a second force harmonic (Fig. S.1F). It is important to note that while the tilted rotor in Fig. S.1B generates net flux over each rotation cycle, the circular rotor in Fig. S.1C does not.

**Viscous energy dissipation by a single rotor.** In Stokes flow, the rate of viscous energy dissipation is proportional to force magnitude squared [24–26]. Thus, the average dissipation due to a single rotor for one period of rotation must be proportional to

$$\langle \mathcal{E} \rangle = \frac{1}{2\pi} \int_0^{2\pi} F(\theta)^2 \, \mathrm{d}\theta = F_o^2 \left[ 1 + \frac{1}{2} \left( \sum_{m=1}^{\infty} \alpha_m^2 + \beta_m^2 \right) \right]. \tag{24}$$

For pure harmonic forcing, *i.e.,* $\alpha_m = \beta_m = \epsilon_m$ is nonzero for only a single value of $m$ and zero otherwise, the viscous energy dissipation rate is proportional to $F_o^2(1 + \epsilon_m^2)$.

**Flow pumping by a single rotor.** A force monopole of strength $\mathbf{F}$, oriented parallel to a no-slip wall at height $h$, pushes fluids at a rate given by $\mathbf{q} = h\mathbf{F}/\pi\eta$ [27, 28]. This is the instantaneous flux. The net flux over one cycle of rotation is given by

$$\langle \mathbf{q} \rangle = \frac{1}{2\pi} \frac{h}{\pi\eta} \int_0^{2\pi} \mathbf{F} \, \mathrm{d}\theta. \tag{25}$$

For a single rotor, $\mathbf{F} = F(\theta)\mathbf{t}$ and $\mathbf{t}$ is the tangent unit vector. Thus, the net flux of a circular rotor parallel to the bounding wall at $z = 0$ is zero for all continuous forcing $F(\theta)$.

### S.2.2 Example of a 1D Ciliary Array

Our goal in this work is to study emergent coordination and fluid pumping in ciliary carpets. However, it is instructive to consider here a simpler example of 1D ciliary array where the coordination is prescribed as in [23, 29, 30], not emergent. We use this example for two purposes: (i) to test the validity of our assumption to ignore hydrodynamic interactions of order $\mathbf{B} \cdot \mathbf{B}$, and (ii) to assess the characteristic scale of fluid pumping due to metachronal coordination.

**Example: 1D array rotors with prescribed metachronal coordination.** By way of background, and to fix ideas for later analysis of emergent coordination, we consider ten circular rotors at distance $d$ apart, each rotating at $\theta_i(t) = \Omega t + i\Delta\theta$, $(i = 1, \ldots, 10)$, where $\Omega$ is a prescribed constant angular speed,

and $\Delta\theta$ is a prescribed phase difference. This produces a prescribed metachronal wave of wavelength $2\pi d/\Delta\theta$. To be consistent with the 2D lattice of rotors considered in the main text and discussed below, the rotors are placed at a height $h = 1$ above a no-slip wall, and we let $a$ be the radius of the bead and $b$ the radius of the rotor trajectory.

**Analogy to Taylor's swimming sheet.** By definition of metachronal coordination (see top row of Fig. S.6), the rotors can be viewed as material points of a sheet undergoing a traveling wave of dimensionless amplitude $A = b/d$, wave number $k = \Delta\theta$, and frequency $\Omega$. This is reminiscent of the classic Taylor's swimming sheet and Blake's envelope model: an impermeable inelastic sheet following a metachronal wave of dimensionless amplitude $A$ will result in net flow that scales with $A^2$ [1,31,32]. Specifically, for a waving sheet with material points following a trajectory of $(x_m, y_m) = (x_o + A\cos(kx+\Omega t), A\sin(kx+\Omega t))$, the net fluid velocity should be $U = A^2/(\Omega/k)$ in the limit of small $k$ [31].

**Force balance and constraint force.** Force balance shows that constraint forces $\mathbf{N}_i$ are needed to balance the viscous drag forces created by the hydrodynamic interactions between all rotors, *i.e.*,

$$\mathbf{F}_i + \mathbf{N}_i - \zeta\left(b\Omega\mathbf{t}_i - \mathbf{v}(\mathbf{r}_i)\right) = 0. \tag{26}$$

Here, $\mathbf{v}(\mathbf{r}_i)$ is the total fluid velocity at rotor $i$ due to all other rotors $j \neq i$. The constraint force $\mathbf{N}_i$ is obtained by taking the inner product of (26) with the normal unit vector $\mathbf{n}_i$,

$$\mathbf{N}_i = -\zeta(\mathbf{n}_i \otimes \mathbf{n}_i)\cdot\mathbf{v}(\mathbf{r}_i) = -\zeta\left(\mathbf{n}_i\cdot\mathbf{v}(\mathbf{r}_i)\right)\mathbf{n}_i, \tag{27}$$

where $\otimes$ denotes the outer tensor product. Given that $\mathbf{F}_i = \zeta b\Omega\mathbf{t}_i$, we compare two approaches: **(i)** we solve for $\mathbf{N}_i$ explicitly by ignoring hydrodynamic interactions of order $\mathbf{B}\cdot\mathbf{B}$ akin to the assumptions made in § S.2.3, that is, by setting $\mathbf{v}(\mathbf{r}_i) = \sum_{j\neq i}\mathbf{B}(\mathbf{r}_i - \mathbf{r_j})\cdot\mathbf{F}_j$; **(ii)** we solve for $\mathbf{N}_i$ implicitly by substituting $\mathbf{v}(\mathbf{r}_i) = \sum_{j\neq i}\mathbf{B}(\mathbf{r}_i - \mathbf{r_j})\cdot(\mathbf{F}_j + \mathbf{N}_i)$ into (27). The latter can be done either in an iterative manner, using the results obtained in (i) as initial guess and performing fixed-point iteration to successively update the constraint forces by solving

$$\mathbf{N}_i^{\text{new}} + \zeta\sum_{j\neq i}\mathbf{B}(\mathbf{r}_i - \mathbf{r_j})\cdot(\mathbf{F}_j + \mathbf{N}_j^{\text{old}}) = 0 \tag{28}$$

until a convergence criterion is met, or by disregarding the iteration superscripts and solve Eq. (28) directly as a linear system.

**Fluid pumping.** To measure fluid pumping, recall that a force monopole of strength $\mathbf{F}$, oriented parallel to a no-slip wall at height $h$, pushes fluids at a rate given by $\mathbf{q} = h\mathbf{F}/\pi\eta$ [27,28]. Using the linearity of Stokes flow, the total instantaneous flux is the sum over all rotors, i.e. $\sum_i \mathbf{q}_i(t)$, where $i$ is the index of the rotor. We calculate the cycle-average flux $\langle\mathbf{q}\rangle$

$$\langle\mathbf{q}\rangle = \frac{1}{2\pi}\frac{1}{N}\frac{h}{\pi\eta}\sum_i\int_0^{2\pi}(\mathbf{F}_i + \mathbf{N}_i)\,\mathrm{d}\theta = -\frac{1}{2\pi}\frac{1}{N}\frac{h}{\pi\eta}\sum_i\int_0^{2\pi}\zeta(\mathbf{n}_i\cdot\mathbf{v}(\mathbf{r}_i(\theta)))\cdot\mathbf{n}_i\,\mathrm{d}\theta. \tag{29}$$

Here, we used the fact that, by construction, an individual rotor cannot produce net flow, *i.e.,* the integral $\int_0^{T_o}\mathbf{F}_j(t)\,\mathrm{d}t$ is zero over one period of the rotor motion. The average flux magnitude $q = \|\mathbf{q}\|$ is set by the magnitude of the constraint force $\|\mathbf{N}_j\| \sim \|\zeta\mathbf{v}_j\|$.

In Fig. S.6, we show the net flux $\|\langle\mathbf{q}\rangle\|$ resulting from approach (i) and (ii) in solid and dashed lines, respectively. On the right panel of Fig. S.6, we normalize the net flux by $Q = hF_d/(\pi\eta)$, where $F_d = \zeta U_d$

Table S.1: **Non-dimensional scales of rotor-based ciliary carpet**

| Parameter | Symbol | Value |
|---|---|---|
| Rotor spacing | $d$ | 1 |
| Rotor forcing | $F_o$ | 1 |
| Fluid viscosity | $\eta$ | 1 |
| Rotor bead radius | $a$ | 0.05 |
| Rotor trajectory radius | $b$ | 0.2 |
| Rotor height | $h$ | 0.1–2 |
| Periodic box length | $L$ | 151 |
| Drag coefficient | $\zeta = 6\pi\eta a$ | $\approx 0.94$ |
| Intrinsic rotor period | $T_o = 2\pi\zeta b/F_o$ | $\approx 1.18$ |
| Characteristic speed | $U_d \sim (\pi b^2/d^2)F_o/(4\pi\eta d)$ | 0.01 |
| Characteristic force | $F_d = \zeta U_d$ | $\approx 0.0094$ |
| Characteristic flux | $Q = hF_d/(\pi\eta)$ | $\approx 0.003h$ |
| Area coverage percentage | $C$ | $0 \sim 1$ |
| Patch wavenumber | $k_{\text{patch}}$ | $0 \sim 9$ |
| Patch displacement parameter | $p_v$ | $0 \sim L/k_{\text{patch}}$ |
| Rotor displacement standard deviation | $\sigma$ | $0 \sim 10d$ |

is a force scale obtained from estimating the velocity $U_d \sim \dfrac{\pi(b/d)^2 F_o}{4\pi\eta d}$ due an individual rotor of nominal force $F_o = 1$ at a distance $d$ away; see Table. S.1. The scaled flux in Fig. S.6(right) collapses for small $b$ and $\Delta\theta$, indicating that the scaling $Q$ is the correct scaling in the limit of small rotor trajectory radius and phase difference.

### S.2.3 Emergent Coordination in Ciliary Carpets

**Equations of motion.** Balance of forces on a cilium $i$ in the fundamental domain dictates that

$$\mathbf{F}_i + \mathbf{N}_i - \zeta\left(b\dot{\theta}_i\mathbf{t}_i - \mathbf{v}(\mathbf{r}_i)\right) = 0, \tag{30}$$

where the subscript $i$ is used to denote the quantity pertaining to cilium $i$. Particularly, the first term in (30) is the active tangential force $\mathbf{F}_i = F_i\mathbf{t}_i = F(\theta_i)\mathbf{t}_i$, and the second term $\mathbf{N}_i = C_i\mathbf{n}_i$ is a normal constraint force that guarantees the bead remains on the desired circular trajectory. Hydrodynamic coupling is accounted for in the last term, which denotes the drag force on the $i$th cilium, and $\mathbf{v}(\mathbf{r}_i)$ is the flow velocity at the position of the $i$-th cilium induced by all other cilia. Neglecting the high order corrections introduced by the wall, the drag coefficient is taken to be $\zeta = 6\pi\eta a$. For a single cilium, the constraint force is identically zero and the intrinsic angular speed $\dot{\theta} = \Omega(\theta) = F(\theta)/\zeta b$ is phase-dependent. For the hydrodynamically-coupled lattice of cilia, the time-evolution of the cilia phase is obtained by taking the inner product of (30) with $\mathbf{t}_i$, leading to a system of coupled differential equations,

$$\dot{\theta}_i = \Omega_i + \frac{1}{b}\mathbf{t}_i \cdot \mathbf{v}(\mathbf{r}_i). \tag{31}$$

Here, $\Omega_i = \Omega(\theta_i) = F(\theta_i)/\zeta b$ refers to the intrinsic angular speed of cilium $i$. We emphasize that all cilia are coupled through the flow velocity $\mathbf{v}$. In our simulations, we normalize this system using the radius of the circular trajectory $d$ as the nominal length scale, the cycle-average force $F_o$ as the nominal force scale, and the viscosity $\eta$ to arrive at a nominal time scale $\eta d^2/F_o$; see Table S.1.

**Fast computation of hydrodynamic interactions.** To close the model in (31), we evaluate the fluid velocity $\mathbf{v}(\mathbf{r}_i)$ at cilium $i$ in the fundamental domain following the procedure described in § S.1.1. Namely, each cilium is a force monopole of strength $\mathbf{F}_i + \mathbf{N}_i$ that induces a fluid velocity according to the singularity solution near a rigid substrate represented by the Blake-Oseen tensor $\mathbf{B}$ in §S.1.1. Considering $N$ cilia in the fundamental domain, the induced velocity at the location of the $i$-th cilium is given by

$$\mathbf{v}_i = \sum_{j=1}^{9N} \mathbf{B}(\mathbf{r}_i - \mathbf{r}_j) \cdot (\mathbf{F}_j + \mathbf{N}_j) \approx \sum_{j=1}^{9N} \mathbf{B}(\mathbf{r}_i - \mathbf{r}_j) \cdot \mathbf{F}_j \approx \sum_{j=1}^{N_s} \mathbf{B}(\mathbf{r}_i - \mathbf{r}_j) \cdot \mathbf{F}_j. \tag{32}$$

Here, we restricted hydrodynamic interactions to the fundamental domain and its eight immediate neighboring domain, hence the sum to $9N$. We omitted the effect of the constraint force, because substituting $\mathbf{N}_i$ by its value from (27), and recalling that $\mathbf{B}$ scales as $1/r^2$, it can be easily seen that the contribution from the constraint forces, which involves $\sum_1^{9N} \mathbf{B} \cdot \mathbf{B}$ scales as the sum of terms of order $1/r^4$, and is thus of higher order (see § S.2.2 for a detailed discussion).

The problem of computing the hydrodynamic interactions, for all $i = 1, \ldots, N$ in the fundamental domain, has a computational complexity of $\mathcal{O}(N^2)$, which can be computationally prohibitive for large $N$, even when considering only the immediate image domains. To reduce the computational cost further, we exploit the quadratic decay of hydrodynamic interactions due to the no-slip substrate at $z = 0$, which implies that truncating hydrodynamic interactions at sufficiently large distances from a focal rotor introduces only a small error in the flow velocity. We thus introduce an "interaction stencil" consisting of $N_s$ force monopoles around each focal force $\mathbf{F}_i$ at $\mathbf{x}_i$ in the fundamental domain; the interaction stencil is represented by a blue square in Fig. S.2B. This simplification reduces the computational complexity from $\mathcal{O}(N^2)$ to $\mathcal{O}(NN_s)$ and allows us to a balance between computational accuracy and cost. In all numerical integration in the main text, we set $N_s = 10$.

**Numerical algorithm for fast temporal integration of cilia phase.** Our approach to accelerate the temporal integration of (31) relies on a key feature in our problem: since all cilia are constrained to move along fixed circular trajectories arranged in a regular square lattice, the interactions between each pair of cilia can be pre-computed and stored in a look-up table that we reference during time integration.

We first discretize each trajectory into $n_\theta$ angular locations as shown in Fig. S.7B. The velocity at the focal cilium $i$ at angular location $p$, induced due to a neighbor cilium $j$ at angular location $q$ is computed using the Blake tensor, and stored offline in a look-up table for future reference. The entries of the look-up table are the components of velocity vectors in the ciliary plane, $\mathbf{v}_{i\leftarrow j}^{p,q}$; they are indexed using the position of the neighboring cilium $j$, relative to the focal cilium $i$, and their discrete angular locations along the trajectories $(p, q)$. The entries corresponding to self-interaction, i.e. $\mathbf{v}_{i\leftarrow i}^{p,q}$, are all set to zero, resulting in a look-up table with $N_s \times n_\theta^2 \times 2$ entries. A step-by-step algorithmic description to construct the velocity look-up table is given in Algorithm 1. It is worth noting that, additional speed gains are achieved by vectorizing sections of the `Matlab` code, wherever possible.

During runtime while integrating equation (31), the pre-computed values of induced velocities are simply looked-up and interpolated from the table based on the relative position of cilia using a classic bi-linear interpolation scheme; see Algorithm 2 for a step-by-step description. In cases where the focal

cilium is close to the boundaries of the primary domain, some cilia in the interaction stencil will be in the image domains (as illustrated in Fig. S.2B). Modulo functions are imposed to identify the copies of such cilia in the primary domain in order to extract their phases. This look-up and interpolation strategy speeds up our program by sidestepping the evaluation of the Blake tensor at each time step, which is computationally more expensive, therefore reduces the constant factor that gets hidden in the $\mathcal{O}$ notation.

**Fluid pumping.** As we integrate the phase dynamics, we calculate the fluid flux at each instant in time following a similar procedure to that in § S.2.2. Namely, we calculate the flux per rotor

$$\mathbf{q}(t) = \frac{1}{N}\frac{h}{\pi\eta}\sum_{j}^{N}\left(\mathbf{F}_j + \mathbf{N}_j\right)(t), \tag{33}$$

The volume of fluid pumped by the carpet up to a time $t$ is simply $\int_0^t \mathbf{q}(\tilde{t})\,\mathrm{d}\tilde{t}$.

# S.3 Synchronization Order Parameters and Kuramoto Ellipse

**Synchronization order parameter fields.** We define the synchronization order parameter fields

$$Y_n(\mathbf{x}, t) = \frac{1}{\rho_c}\sum_{j} \mathrm{e}^{\mathrm{i}n\phi_j}\delta(\mathbf{x} - \mathbf{x}_j), \tag{34}$$

where $\phi_j$ is the phase of the $j$th cilium, related to $\theta_j$ via a nonlinear transformation described in § S.4. By definition, $Y_1$ is the Kuramoto order field, and $Y_2$ the nematic order field. The spatial average of $Y_1$ over the doubly-periodic domain leads to the Kuramoto order parameter $P = |\langle Y_1\rangle| = \left|\int_{-L/2}^{L/2}\int_{-L/2}^{L/2} Y_1(x,y)\,\mathrm{d}x\,\mathrm{d}y\right|$; values of $P$ near zero indicate phase disorder while values near one correspond to phase synchrony [33]. For each value of $n$, the quantity $|\langle Y_n\rangle| = 1$ captures a different kind of phase order. For instance, $|\langle Y_2\rangle| = 1$ captures anti-phase synchrony, $|\langle Y_3\rangle| = 1$ captures a Mercedes star-like arrangement of rotors around the phase circle, and so on.

**The Kuramoto ellipse.** We introduce the "Kuramoto ellipse" as a metric to quantify the appearance of spatial wave patterns. Starting from the discrete particle model, we compute the Kuramoto order field [33] at the location $\mathbf{x}_j$ of a cilium $j$ by averaging over all cilia in a local neighborhood of $j$,

$$Y_1(\mathbf{x}_j) = \frac{1}{\rho_c}\sum_{\ell\in\mathcal{N}(j)} e^{i\phi_\ell}. \tag{S1}$$

Here, we choose $\mathcal{N}(j)$ to contain one shell of neighbors around cilium $j$. We repeat this at the location of each cilium on the grid to estimate the Kuramoto order field $Y_1(\mathbf{x})$ from discrete cilia simulations. Next, we draw straight lines starting from the origin of the fundamental domain at angles $\alpha \in [0, 2\pi)$, and compute the average magnitude of order parameter along that direction:

$$P_\alpha = \left|\int_0^{L/2} Y_1(s\cos\alpha, s\sin\alpha)\,\mathrm{d}s\right|. \tag{S3}$$

Note that $P_\alpha$ is the absolute value of (a constrained version of) the Radon transform of the 2D field $Y_1(\mathbf{x})$ [34]. We use the polar coordinate representation $(\alpha, P_\alpha)$ to obtain the data points indicated by the green dots in Fig. S.8C. We apply a Principal Component Analysis to these data points to fit, what

we call, the *Kuramoto ellipse*, whose major and minor axes correspond to the first and second principle components, respectively.

Fig. S.8 shows the Kuramoto ellipse corresponding to two snapshots taken from an isotropic state (top row) and a synthetically-generated wave state (bottom row). In the isotropic state, $(\alpha, P_\alpha)$ are distributed in an almost circular fashion around the origin, indicating lack of spatial order. In the wave state, since spatial order is maximum along the direction of wave orientation, the ellipse stretches out in that direction. We refer to the eccentricity of the ellipse as the *Kuramoto eccentricity*, and the inclination of the first principal component to the horizontal as the *Kuramoto angle*. The Kuramoto eccentricity is a measure of the degree of coherence of waves, while the inclinations of the first and second principal component give us the directions of wave orientation and propagation, respectively.

To further probe the meaning of the Kuramoto eccentricity, we prescribe a phase field of $\theta = mx/L$, which will produce standing waves in the $x-$direction with wavenumber $m$; see Fig. S.9A. In this set up, we can compute the quantity $P_\alpha(\alpha) = |\int_0^{L/2} Y_1(s\cos\alpha, s\sin\alpha)\,\mathrm{d}s|$ analytically to be $P_\alpha(\alpha) = 2|\sec\alpha\sin((m\cos\alpha)/4)|/m$. Performing Principal Component Analysis (PCA) for $(\alpha, P_\alpha)$ in polar coordinates, the Kuramoto eccentricity can be easily obtained; see Fig. S.9B,C. We find that the Kuramoto eccentricity is generally increasing as a function of the wavenumber $m$ but with some small oscillations. In the synchronized state, where wavenumber $m = 0$, the eccentricity is zero. As the wavenumber increases, the eccentricity quickly rise to a value near 1. In the limit of infinite wavenumber, the theoretical eccentricity is 1. Note that in discrete numerical computations, eccentricity for wavenumbers similar or greater than the rotor distance $\pi/d$ will be smaller due to aliasing effects.

# S.4 Continuum Theory of Synchronization in Ciliary Carpets

We seek to develop a continuum theory for cilia coordination. We first introduce the order parameter fields that describe synchronization in the continuous limit and derive the governing equations of motion. We then discuss the relation between these order parameters, the ciliary forces, and fluid flows.

**Synchronization order parameter fields.** Following [35], we propose to derive equations of motion governing the synchronization order parameter fields

$$Y_n(\mathbf{x}, t) = \lim_{N\to\infty} \frac{1}{\rho_c} \sum_j^N \mathrm{e}^{\mathrm{i}n\phi_j} \delta(\mathbf{x} - \mathbf{x}_j). \tag{35}$$

Hereafter, we drop the $\lim_{N\to\infty}$ for notational simplicity.

**Nonlinear phase transformation.** A priori the choice of the phase $\phi_j$ is not unique. For example, it can be $\theta_j$ or any smooth non-decreasing function of $\theta_j$. We fix this freedom by requiring that the phase of an unperturbed cilium, that is a cilium in a quiescent background fluid with $\mathbf{v} = 0$, obeys

$$\dot{\phi}_j = \Omega_0, \tag{36}$$

where $\Omega_0 = 2\pi/T_0$ is a constant. Here, $T_0 = \int_0^{2\pi} \mathrm{d}\bar{\theta}/\Omega(\bar{\theta})$ is the beat period of the cilium in a quiescent background fluid. This definition ensures that $\phi(\theta + 2\pi) = \phi(\theta)$ and implies a mapping

$$\phi_j(\theta_j) = \Omega_0 \int_0^{\theta_j} \frac{\mathrm{d}\bar{\theta}}{\Omega(\bar{\theta})}, \tag{37}$$

from the angular position $\theta_j$ of the cilium along its beat cycle onto its phase $\phi_j$. This mapping is unique as long as the cilium does not reverse its direction of motion. In the case of phase independent driving,

that is, when $F(\theta_j)$ = constant, $\phi_j$ and $\theta_j$ are identical. In all other cases $\phi_j$ and $\theta_j$ are distinct, as shown in Fig. S.11 for representative examples of the first two force harmonics. Importantly, this phase definition implies that in a system where the cilia phases $\phi_j$ are distributed uniformly on the unit circle, the total force cilia exert on the fluid, and thus the induced flow field, vanishes. We will call this state phase isotropic.

**Derivation of equations of motion.** We substitute (37) into (31); we arrive at the equations of motion written in terms of $\phi_j$ in the general case where the flow field is not necessarily zero $\mathbf{v} \neq 0$,

$$\dot{\phi}_j = \Omega_0 + \frac{\Omega_0}{b\Omega_j}\mathbf{t}_j \cdot \mathbf{v}(\mathbf{r}_j). \tag{38}$$

Taking the time derivative of (34) and using (38), we arrive at the equations of motion for the moments $Y_n$

$$\dot{Y}_n(\mathbf{x}) = \frac{1}{\rho_c}\sum_j ine^{in\phi_j}\delta(\mathbf{x}-\mathbf{x}_j)\left(\Omega_0 + \frac{\Omega_0}{b\Omega_j}\mathbf{t}_j \cdot \mathbf{v}(\mathbf{x}_j + b\mathbf{n}_j)\right). \tag{39}$$

We next expand the induced velocity $\mathbf{v}(\mathbf{x}_j + b\mathbf{n}_j) = \mathbf{v}(\mathbf{x}_j) + b\nabla\mathbf{v}(\mathbf{x}_j)\cdot\mathbf{n}_j + \mathcal{O}(b^2)$ about the trajectory center $\mathbf{x}_j$ and arrive at

$$\dot{Y}_n(\mathbf{x}) = in\Omega_0 Y_n(\mathbf{x}) + \frac{in\Omega_0}{\rho_c}\sum_j e^{in\phi_j}\delta(\mathbf{x}-\mathbf{x}_j)\frac{\mathbf{t}_j}{b\Omega_j}\cdot\left(\mathbf{v}(\mathbf{x}_j) + b\nabla\mathbf{v}(\mathbf{x}_j)\cdot\mathbf{n}_j + \mathcal{O}(b^2)\right). \tag{40}$$

Considering $b/d \ll 1$, dropping higher order terms and rearranging, we get

$$\dot{Y}_n(\mathbf{x}) = in\Omega_0 Y_n(\mathbf{x}) + \frac{in\Omega_0}{\rho_c}\sum_j e^{in\phi_j}\delta(\mathbf{x}-\mathbf{x}_j)\left[\mathbf{v}(\mathbf{x}_j)\cdot\frac{\mathbf{t}_j}{b\Omega_j} + \nabla\mathbf{v}(\mathbf{x}_j) : \frac{\mathbf{t}_j\otimes\mathbf{n}_j}{\Omega_j}\right], \tag{41}$$

where ‘:’ denotes tensor contraction. Next, it is useful to define

$$\mathbf{a}(\phi) = \frac{\mathbf{t}(\phi)}{b\Omega(\phi)}, \qquad \mathbf{B}(\phi) = \frac{\mathbf{t}(\phi)\otimes\mathbf{n}(\phi)}{\Omega(\phi)}, \tag{42}$$

where $\mathbf{a}(\phi)$ is a vector, $\mathbf{B}(\phi)$ is a second order tensor. Their complex Fourier series may be written in terms of $\phi$ as $\mathbf{a}(\phi) = \sum_{m=-\infty}^{\infty} \widetilde{\mathbf{a}}_m e^{im\phi}$, $\mathbf{B}(\phi) = \sum_{m=-\infty}^{\infty} \widetilde{\mathbf{B}}_m e^{im\phi}$, where

$$\widetilde{\mathbf{a}}_m = \frac{1}{2\pi}\int_0^{2\pi}\mathbf{a}(\phi)e^{-im\phi}\,\mathrm{d}\phi, \qquad \widetilde{\mathbf{B}}_m = \frac{1}{2\pi}\int_0^{2\pi}\mathbf{B}(\phi)e^{-im\phi}\,\mathrm{d}\phi. \tag{43}$$

Substituting this into equation (41), we get

$$\dot{Y}_n(\mathbf{x}) = in\Omega_0 Y_n(\mathbf{x}) + \frac{in\Omega_0}{\rho_c}\sum_j e^{in\phi_j}\delta(\mathbf{x}-\mathbf{x}_j)\left[\mathbf{v}(\mathbf{x}_j)\cdot\sum_m \widetilde{\mathbf{a}}_m e^{im\phi_j} + \nabla\mathbf{v}(\mathbf{x}_j) : \sum_m \widetilde{\mathbf{B}}_m e^{im\phi_j}\right]. \tag{44}$$

Exchanging the order of the two summations and using the substitution property of the Dirac delta, $\mathbf{v}(\mathbf{x}_j)\delta(\mathbf{x}-\mathbf{x}_j) = \mathbf{v}(\mathbf{x})\delta(\mathbf{x}-\mathbf{x}_j)$, we finally arrive at

$$\dot{Y}_n(\mathbf{x}) = in\Omega_0\Big[Y_n(\mathbf{x}) + \sum_m\left(\widetilde{\mathbf{a}}_m\cdot\mathbf{v}(\mathbf{x}) + \widetilde{\mathbf{B}}_m : \nabla\mathbf{v}(\mathbf{x})\right)Y_{n+m}(\mathbf{x})\Big], \tag{45}$$

which capture the phase dynamics of the system.

These equations provide a coupled set of linear partial differential equations that, together with (16) and (17), describe the dynamical evolution of the macroscopic variables $Y_n(\mathbf{x}, t)$.

**Expressing the ciliary force density in terms of flow velocity and synchronization fields.** We next derive an expression for $\mathbf{f}(\mathbf{x})$ in terms of the coarse-grained variables $\mathbf{v}(\mathbf{x})$ and $Y_n(\mathbf{x})$. We redefine $\mathbf{f}(\mathbf{x})$ from (6) as follows

$$\mathbf{f}(\mathbf{x}) \;=\; \lim_{N\to\infty}\sum_{j}^{N}\delta(\mathbf{x}-\mathbf{r}_j)(\mathbf{F}_j+\mathbf{N}_j), \tag{46}$$

Using (30) and (31), and dropping the $\lim_{N\to\infty}$ for notational simplicity, we get

$$\mathbf{f}(\mathbf{x}) \;=\; \sum_{j}\delta(\mathbf{x}-\mathbf{r}_j)(\zeta b\Omega_j\mathbf{t}_j-\zeta(\mathbf{n}_j\otimes\mathbf{n}_j)\cdot\mathbf{v}(\mathbf{r}_j)), \tag{47}$$

Expanding this expression about $\mathbf{x}_j$ and keeping terms up to $\mathcal{O}\left(b^2\right)$ yields

$$\mathbf{f}(\mathbf{x}) = \boldsymbol{\mathcal{F}}(\mathbf{x}) + \nabla\cdot\boldsymbol{\Sigma}(\mathbf{x}), \tag{48}$$

where the surface force density exerted by the continuous ciliary layer is

$$\boldsymbol{\mathcal{F}}(\mathbf{x}) = \sum_{j}\delta(\mathbf{x}-\mathbf{x}_j)\zeta(b\Omega_j\mathbf{t}_j-(\mathbf{n}_j\otimes\mathbf{n}_j)\cdot\mathbf{v}(\mathbf{x}_j)), \tag{49}$$

and the surface stress density exerted by the ciliary layer is

$$\boldsymbol{\Sigma}(\mathbf{x}) = \sum_{j}\delta(\mathbf{x}-\mathbf{x}_j)\zeta b\mathbf{n}_j\otimes(b\Omega_j\mathbf{t}_j-(\mathbf{n}_j\otimes\mathbf{n}_j)\cdot\mathbf{v}(\mathbf{x}_j)). \tag{50}$$

For notational convenience, we introduce,

$$\mathbf{c} = b\Omega_j\mathbf{t}_j, \qquad \mathbf{D} = \mathbf{n}_j\otimes\mathbf{n}_j, \qquad \mathbf{E} = b\Omega_j\mathbf{n}_j\otimes\mathbf{t}_j, \qquad \mathbf{G} = 2\mathbf{n}_j\otimes\mathbf{n}_j\otimes\mathbf{n}_j, \tag{51}$$

where $\mathbf{c}=\mathbf{c}(\phi)$ is a vector, $\mathbf{D}=\mathbf{D}(\phi)$ and $\mathbf{E}=\mathbf{E}(\phi)$ are second order tensors, and $\mathbf{G}=\mathbf{G}(\phi)$ is a third order tensor. Next, we write their Fourier series expansions,

$$\mathbf{c} = \sum_{m=-\infty}^{\infty}\widetilde{\mathbf{c}}_m e^{im\phi_j}, \quad \mathbf{D} = \sum_{m=-\infty}^{\infty}\widetilde{\mathbf{D}}_m e^{im\phi_j}, \quad \mathbf{E} = \sum_{m=-\infty}^{\infty}\widetilde{\mathbf{E}}_m e^{im\phi_j}, \quad \mathbf{G} = \sum_{m=-\infty}^{\infty}\widetilde{\mathbf{G}}_m e^{im\phi_j}. \tag{52}$$

Here $\widetilde{\mathbf{c}}_m$, $\widetilde{\mathbf{D}}_m$, $\widetilde{\mathbf{E}}_m$, and $\widetilde{\mathbf{G}}_m$ are the associated Fourier coefficients and follow from formulae similar to those in (43). With this

$$\boldsymbol{\mathcal{F}}(\mathbf{x}) = \rho_c\sum_{m}\zeta\left(\widetilde{\mathbf{c}}_m-\widetilde{\mathbf{D}}_m\cdot\mathbf{v}(\mathbf{x})\right)Y_m, \qquad \boldsymbol{\Sigma}(\mathbf{x}) = \rho_c\sum_{m}\zeta b\left(\widetilde{\mathbf{E}}_m-\widetilde{\mathbf{G}}_m\cdot\mathbf{v}(\mathbf{x})\right)Y_m, \tag{53}$$

and finally

$$\mathbf{f}(\mathbf{x}) = \rho_c\zeta\sum_{m}\left(\widetilde{\mathbf{c}}_m-\widetilde{\mathbf{D}}_m\cdot\mathbf{v}(\mathbf{x})\right)Y_m + b\nabla\cdot\left((\widetilde{\mathbf{E}}_m-\widetilde{\mathbf{G}}_m\cdot\mathbf{v}(\mathbf{x}))Y_m\right), \tag{54}$$

which is the cilia generated forcing on the system. The flow velocity $\mathbf{v}$ can be calculated by solving (16), together with (17), which is a linear in $\mathbf{f}$.

# S.5 Linear Stability Analysis in the Continuum Theory

We use the continuum theory developed above to investigate the stability of two spatially homogeneous states that do not pump fluid: (i) the isotropic steady state, and (ii) the fully synchronized steady state.

**Spatially-uniform isotropic state.** The spatially-homogeneous isotropic steady state of the ciliary system is defined by $Y_m = 0$, for all non-zero $m$. In this case, the force $\mathbf{f}$ that the cilia collectively exert on the fluid vanishes. Thus no fluid flow is induced and the individual cilia act as if they were independent.

**Spatially-uniform isotropic state.** The fully synchronized steady state is the state in which the phase of all cilia is the same, i.e., $\phi_j = \phi$ for all $j$. In this case, $\nabla \mathbf{v} = 0$ and $\mathbf{v}$ is parallel to the instantaneous direction of motion of all cilia such that (41) simplifies to

$$\dot{Y}_n = in\left(1 + \frac{v(\phi)}{b\Omega(\phi)}\right)\Omega_0 Y_n, \tag{55}$$

where $v = \|\mathbf{v}\| = \mathbf{v}\cdot\mathbf{t}$. Thus, the fully synchronized state is a periodic steady state. The same conclusion can also be arrived at directly from (38). Note that in the case of an $M$-fold symmetric forcing function, the system admits $M$ additional spatially homogeneous periodic steady states, as can be directly seen from (38). Hereafter, we make no further comment on these special cases.

### S.5.1 Stability of the Isotropic State

We investigate the linear stability of the isotropic state subject to small perturbations. For notational convenience, we use the notation $X^*$ to indicate the steady state value of a quantity $X$ and $\delta X$ to indicate a small perturbation away from the steady state. For instance $Y_n = Y_n^* + \delta Y_n$, $\mathbf{f}(\mathbf{x}) = \mathbf{f}^*(\mathbf{x}) + \delta\mathbf{f}(\mathbf{x})$, and $\mathbf{v}(\mathbf{x}) = \mathbf{v}^*(\mathbf{x}) + \delta\mathbf{v}(\mathbf{x})$.

For the isotropic state, we have $Y_0^* = 1$, which is the constant cilia surface density, and $Y_n^* = 0$ for all $n \neq 0$. Also, $\mathbf{f}^*(\mathbf{x})$ and $\mathbf{v}^*(\mathbf{x})$ are identically zero. Substituting into (45) and (54), respectively, we get to linear order,

$$\delta\dot{Y}_n(\mathbf{x}) = in\Omega_0\left(\delta Y_n + \widetilde{\mathbf{a}}_{-n}\cdot\delta\mathbf{v}(\mathbf{x}) + \widetilde{\mathbf{B}}_{-n} : \nabla\delta\mathbf{v}(\mathbf{x})\right). \tag{56}$$

Expanding (54), to linear order again, we find

$$\delta\mathbf{f}(\mathbf{x}) = \rho_c\zeta\left(-\widetilde{\mathbf{D}}_0\cdot\delta\mathbf{v} - b\nabla\cdot\widetilde{\mathbf{G}}_0\cdot\delta\mathbf{v} + \sum_m \widetilde{\mathbf{c}}_m\delta Y_m + b\nabla\cdot\widetilde{\mathbf{E}}_m\delta Y_m\right) \tag{57}$$

We next write equations (56) and (57) in Fourier space,

$$\delta\hat{\dot{Y}}_n(\mathbf{k}) = in\Omega_0\delta\hat{Y}_n(\mathbf{k}) + \left(\widetilde{\mathbf{a}}_{-n} + i\widetilde{\mathbf{B}}_{-n}\cdot\mathbf{k}\right)\cdot\delta\hat{\mathbf{v}}(\mathbf{k}), \tag{58}$$

and

$$\delta\hat{\mathbf{f}}(\mathbf{k}) = -\rho_c\zeta(\widetilde{\mathbf{D}}_0 + ib\mathbf{k}\cdot\widetilde{\mathbf{G}}_0)\cdot\delta\hat{\mathbf{v}}(\mathbf{k}) + \rho_c\zeta\sum_m\left(\widetilde{\mathbf{c}}_m + ib\mathbf{k}\cdot\widetilde{\mathbf{E}}_m\right)\delta\hat{Y}_m(\mathbf{k}), \tag{59}$$

and substitute (59) into (16). After some rearranging we arrive at

$$\left[\mathbf{I} + \rho_c\zeta\hat{\mathbf{K}}\cdot\left(\widetilde{\mathbf{D}}_0 + ib\mathbf{k}\cdot\widetilde{\mathbf{G}}_0\right)\right]\cdot\delta\hat{\mathbf{v}}(\mathbf{k}) = \rho_c\zeta\hat{\mathbf{K}}\cdot\sum_m\left(\widetilde{\mathbf{c}}_m + ib\mathbf{k}\cdot\widetilde{\mathbf{E}}_m\right)\delta\hat{Y}_m(\mathbf{k}). \tag{60}$$

Without further approximations, to linear order, we can write $\delta\hat{\mathbf{v}}(\mathbf{k}) = \sum_m \hat{\boldsymbol{\nu}}_m(\mathbf{k})\delta\hat{Y}_m(\mathbf{k})$ where, $\hat{\boldsymbol{\nu}}_m(\mathbf{k})$ is a vector-valued function,

$$\hat{\boldsymbol{\nu}}_m(\mathbf{k}) = \left[\mathbf{I} + \rho_c\zeta\hat{\mathbf{K}}\cdot(\widetilde{\mathbf{D}}_0 + ib\mathbf{k}\cdot\widetilde{\mathbf{G}}_0)\right]^{-1}\cdot\rho_c\zeta\hat{\mathbf{K}}\cdot\sum_m\left(\widetilde{\mathbf{c}}_m + ib\mathbf{k}\cdot\widetilde{\mathbf{E}}_m\right). \tag{61}$$

Substituting this expression for $\delta\hat{\mathbf{v}}$ in (58), we arrive at

$$\delta\dot{\hat{Y}}_n(\mathbf{k}) = in\Omega_0 \left( \delta\hat{Y}_n(\mathbf{k}) + (\widetilde{\mathbf{a}}_{-n} + i\widetilde{\mathbf{B}}_{-n} \cdot \mathbf{k}) \cdot \sum_m \hat{\boldsymbol{\nu}}_m(\mathbf{k}) \delta\widetilde{Y}_m(\mathbf{k}) \right) = \sum_m \hat{L}_{nm}(\mathbf{k}) \delta\hat{Y}_m(\mathbf{k}), \tag{62}$$

where

$$\hat{L}_{nm}(\mathbf{k}) = in\Omega_0 \left( \delta_{nm} + (\widetilde{\mathbf{a}}_{-n} + i\widetilde{\mathbf{B}}_{-n} \cdot \mathbf{k}) \cdot \boldsymbol{\nu}_m(\mathbf{k}) \right), \tag{63}$$

is a second order tensor that couples the perturbations in the order parameter fields. The largest eigenvalue $\gamma(\mathbf{k})$ of $\hat{\mathbf{L}}(\mathbf{k})$ is the growth rate of the fastest growing eigenvector of the system. The sign of the real part of $\gamma(\mathbf{k})$ determines the overall stability of the isotropic steady state.

To evaluate (63) numerically, we truncate the summation in (61) retaining only the terms $m = -5$ through $m = +5$. This results in the coupling matrix $\hat{\mathbf{L}}(\mathbf{k})$ (with entries $\hat{L}_{nm}$) having dimension $11 \times 11$. The largest eigenvalue gives the growth rate $\gamma(\mathbf{k})$ of the system.

### S.5.2 Stability of the Synchronized State

In the fully synchronized state, all cilia beat in-phase and $\phi_j = \phi^*$ for all $j$. This also implies that $\theta_j = \theta^*$ and $\mathbf{v}(\mathbf{x}_j) = \mathbf{v}^*$ for all $j$ and thus the system is in steady state, see Eq (31). The angular speed at steady state is $\dot{\theta}^* = \Omega^* + \mathbf{t}^* \cdot \mathbf{v}^*/b$. Note that the intrinsic angular speed $\Omega^* = \Omega(\theta^*)$ is a periodic function of the angle $\theta^*$. We ask whether the fully synchronized state is linearly stable. As in the previous section, the superscript $()^*$ denotes quantities at the steady state, and the prefix $\delta$ indicates the perturbation.

We start from the observation that in the fully synchronized state, the velocity gradient is identically zero

$$\nabla\mathbf{v}|_* = 0, \tag{64}$$

and the order parameters take the form

$$Y_m^* = e^{im\phi} = (Y_1^*)^m. \tag{65}$$

Substituting (64) into (54) gives the force density in the fully synchronized state

$$\mathbf{f}^* = \rho_c\zeta \sum_m \left( \widetilde{\mathbf{c}}_m - \widetilde{\mathbf{D}}_m \cdot \mathbf{v}^* \right) Y_m^*, \tag{66}$$

and the fluid velocity

$$\mathbf{v}^* = \frac{\rho_c\zeta h}{\eta} \left( \mathbf{I} + \frac{\rho_c\zeta h}{\eta} \sum_m \widetilde{\mathbf{D}}_m Y_m^* \right)^{-1} \cdot \sum_m \widetilde{\mathbf{c}}_m Y_m^*. \tag{67}$$

We next note that given Eq. (65), perturbations $\delta Y_m$ around the fully synchronized steady state can be expressed in terms of $\delta Y_1$ using the relation

$$\delta Y_m = m Y_{m-1}^* \delta Y_1. \tag{68}$$

With this, to linear order, (45) becomes

$$\delta\dot{Y}_1 = i\Omega_0 \left[ \delta Y_1 + \sum_m \left( \widetilde{\mathbf{a}}_m \cdot \delta\mathbf{v} + \widetilde{\mathbf{B}}_m : \nabla\delta\mathbf{v} \right) Y_{m+1}^* + (m+1)\widetilde{\mathbf{a}}_m \cdot \mathbf{v}^* Y_m^* \delta Y_1 \right]. \tag{69}$$

Similarly, taking variations of (54) gives

$$\delta\mathbf{f} = \rho_c\zeta \sum_m \left(\widetilde{\mathbf{c}}_m - \widetilde{\mathbf{D}}_m \cdot \mathbf{v}^*\right) \delta Y_m - \widetilde{\mathbf{D}}_m \cdot \delta\mathbf{v} Y_m^* \\ + b\nabla \cdot \widetilde{\mathbf{E}}_m \delta Y_m - b\nabla \cdot \widetilde{\mathbf{G}}_m \cdot \delta\mathbf{v} Y_m^*, \tag{70}$$

In Fourier space, (69) and (70) become

$$\delta\dot{\hat{Y}}_1 = i\Omega_0 \left[\delta\hat{Y}_1 + \sum_m \left(\widetilde{\mathbf{a}}_m + i\widetilde{\mathbf{B}}_m \cdot \mathbf{k}\right) \cdot \delta\hat{\mathbf{v}} Y_{m+1}^* + (m+1)\widetilde{\mathbf{a}}_m \cdot \mathbf{v}^* Y_m^* \delta\hat{Y}_1\right], \tag{71}$$

and

$$\delta\hat{\mathbf{f}} = \rho_c\zeta \sum_m \left(\widetilde{\mathbf{c}}_m - \widetilde{\mathbf{D}}_m \cdot \mathbf{v}^*\right) m Y_{m-1}^* \delta\hat{Y}_1 - \widetilde{\mathbf{D}}_m \cdot \delta\hat{\mathbf{v}} Y_m^* \\ + ib\mathbf{k} \cdot \widetilde{\mathbf{E}}_m m Y_{m-1}^* \delta\hat{Y}_1 - ib\mathbf{k} \cdot \widetilde{\mathbf{G}}_m \cdot \delta\hat{\mathbf{v}} Y_m^*. \tag{72}$$

Substituting (72) into (16) we obtain an expression for the velocity perturbation

$$\delta\hat{\mathbf{v}} = \boldsymbol{\nu}\delta\hat{Y}_1 \tag{73}$$

where the vector $\boldsymbol{\nu}$ is given by

$$\boldsymbol{\nu} = \left[\mathbf{I} + \rho_c\zeta\hat{\mathbf{K}} \cdot \sum_m \left(\widetilde{\mathbf{D}}_m + ib\mathbf{k} \cdot \widetilde{\mathbf{G}}_m\right) Y_m^*\right]^{-1} \cdot \left(\rho_c\zeta\hat{\mathbf{K}} \cdot \sum_n n \left(\widetilde{\mathbf{c}}_n - \widetilde{\mathbf{D}}_n \cdot \mathbf{v}^* + ib\mathbf{k} \cdot \widetilde{\mathbf{E}}_n\right) Y_{n-1}^*\right). \tag{74}$$

Finally substituting this back into equation (71) we arrive at the linearized equation of motion

$$\delta\dot{\hat{Y}}_1 = \hat{L}(t)\delta\hat{Y}_1 \tag{75}$$

where

$$\hat{L}(t) = i\Omega_0 \left(1 + \sum_m \left(\widetilde{\mathbf{a}}_m + i\widetilde{\mathbf{B}}_m \cdot \mathbf{k}\right) \cdot \boldsymbol{\nu} \cdot Y_{m+1}^* + (m+1)\widetilde{\mathbf{a}}_m \cdot \mathbf{v}^* \cdot Y_m^*\right). \tag{76}$$

It is worth noting that $\hat{L}$ here is a complex scalar, while it is a complex matrix in the linearized equations about the isotropic state (62). This is a direct consequence of (65), which states that the dynamics of the system in the fully synchronized state can be captured using $Y_1$ alone without the need for higher moments. Eq. (75) is a first order ODE that describes the time evolution of the perturbation $\delta\hat{Y}_1(\mathbf{k}, t)$; it admits the solution

$$\delta\hat{Y}_1(\mathbf{k}, t = \tau) = \delta\hat{Y}_1(\mathbf{k}, t = 0) e^{\int_0^\tau \hat{L}(t)\,\mathrm{d}t}. \tag{77}$$

Equation (77) gives the growth of the perturbation up to time $t = \tau$. Since the fully synchronized state is a periodic steady state, we are specifically interested in the growth of the perturbation over one beat cycle, $T^* = \int_0^{2\pi} \mathrm{d}\phi/\phi^*$. To this end, we calculate the Lyapunov exponent, $\mu(\mathbf{k})$, which is given by

$$\mu(\mathbf{k}) = \frac{1}{T^*}\mathrm{Real}\left(\int_0^{T^*} \hat{L}(t)\,\mathrm{d}t\right). \tag{78}$$

Finally, we use the transformation $\mathrm{d}t = \mathrm{d}\phi/\dot{\phi}^*$ to get

$$\mu(\mathbf{k}) = \frac{1}{T^*}\mathrm{Real}\left(\int_0^{2\pi} \frac{\hat{L}(t)}{\dot{\phi}^*}\,\mathrm{d}\phi\right). \tag{79}$$

The steady state is linearly stable if the Lyapunov exponent $\mu(\mathbf{k}) < 0$, critically stable for $\mu(\mathbf{k}) = 0$, and linearly unstable when $\mu(\mathbf{k}) > 0$.

## S.6 Heterogeneity in Ciliary Carpets

In order to study the effect of tissue-level heterogeneity on phase coordination in ciliary carpets, we introduce abstract representation of tissue organization parameters in the rotor-based model. Inspired by [36], we introduce four parameters. First we define the coverage fraction $C \in (0,1)$, which represents the ratio between the area covered by cilia and the total area $L^2$ of the fundamental domain. Second, we consider that the cilia appear in several regular patches and we define the patch wavenumber $k_{\text{patch}} \in \mathbb{Z}$, which represents the number of patches in the $x$- and $y$-directions. Third, we allow the patches to occupy non-regular locations in the fundamental domain, by introducing a patch misalignment scale $p_v \in (0,1)$ with a non-negative rotor displacement standard deviation parameter $\sigma$ that controls the randomness built into our simulated patches.

To implement these parameters numerically and compute the positions in the fundamental domain that are covered by cilia, we design a Boolean function of $(x,y)$ that returns true if and only if a rotor is present at that location. We start from a 1D triangular-wave function $\mathcal{T}(x;a)$, parameterized to vary periodically from $-1$ to 1 with a period of 1, and apex at $x=a$ in each wavelength

$$\mathcal{T}(x;a) = \begin{cases} \text{mod}(x+1,2)/a - 1 & \text{mod }(x+1,2) \leq 2a \\ 1 - (\text{mod}(x+1,2) - 2a)/(1-a) & \text{mod }(x+1,2) > 2a \end{cases}, \tag{80}$$

The piecewise linearity of the triangular-wave allows us to obtain an arbitrary coverage ratio $L_C$ by setting a function to return true if and only if $\mathcal{T}(x;a)$ is above $1-2L_C$ (see Fig. S.12A). We generalize this one-dimensional construction to two-dimensions by combining two 1D functions using the unit norm separable function $f(x,y) = \min(f(x), f(y))$. Namely, we get

$$\mathcal{T}_{\text{2D}}(x,y;a_x,a_y) = \min\left[\mathcal{T}\left(\frac{k_{\text{patch}}x}{L};a_x\right), \mathcal{T}\left(\frac{k_{\text{patch}}y}{L};a_y\right)\right], \tag{81}$$

where we re-parameterize $x$ and $y$ by the patch wavelength $L/k_{\text{patch}}$, and introduce independent apex position parameter $a_x, a_y \sim \mathcal{U}(0, p_v L/k_{\text{patch}})$ from a uniform distribution with an upper bound controlled by the patch displacement parameter $p_v$ (Fig. S.12B). To ensure that the area fraction of the periodic domain covered by cilia is $C$, we set $L_C = \sqrt{C}$ and test if $\mathcal{T}_{\text{2D}}(x,y)$ is above $1-2L_C$ just like in the one-dimensional case (Fig. S.12C). Lastly, to randomize rotor displacement inside each patch, we add Gaussian noise $\eta_x, \eta_y \sim \mathcal{N}(0,\sigma)$ to the position variables $x, y$ (Fig. S.12D).

# References


[1] Blake J. Infinite models for ciliary propulsion. Journal of Fluid Mechanics. 1971;49(2):209–222.

[2] Gimbutas Z, Greengard L, Veerapaneni S. Simple and efficient representations for the fundamental solutions of Stokes flow in a half-space. Journal of Fluid Mechanics. 2015;776.

[3] Yan W, Shelley M. Universal image systems for non-periodic and periodic Stokes flows above a no-slip wall. Journal of Computational Physics. 2018;375:263–270.

[4] Yan W, Blackwell R. Kernel aggregated fast multipole method. Advances in Computational Mathematics. 2021;47(5):1–27.

[5] Hasimoto H. On the periodic fundamental solutions of the Stokes equations and their application to viscous flow past a cubic array of spheres. J Fluid Mech. 1959;5(02):317–328.

[6] Masoud H, Shelley MJ. Collective surfing of chemically active particles. Physical Review Letters. 2014;112(12):128304.

[7] Gao T, Blackwell R, Glaser MA, Betterton MD, Shelley MJ. Multiscale polar theory of microtubule and motor-protein assemblies. Physical Review Letters. 2015;114(4):048101.

[8] Purcell EM. Life at low Reynolds number. American Journal of Physics. 1977;45(1):3–11.

[9] Jung I, Powers TR, Valles Jr JM. Evidence for two extremes of ciliary motor response in a single swimming microorganism. Biophysical Journal. 2014;106(1):106–113.

[10] Woolley DM. Flagellar oscillation: a commentary on proposed mechanisms. Biological Reviews. 2010;85(3):453–470.

[11] Chioccioli M, Feriani L, Nguyen Q, Kotar J, Dell SD, Mennella V, et al. Quantitative high-speed video profiling discriminates between DNAH11 and HYDIN variants of primary ciliary dyskinesia. American journal of respiratory and critical care medicine. 2019;199(11):1436–1438.

[12] Chioccioli M, Feriani L, Nguyen Q, Kotar J, Dell S, Mennella V, et al. A How-To guide to: Quantitative high-speed video profiling to discriminate between variants of primary ciliary dyskinesia. bioRxiv. 2019;p. 614966.

[13] Vilfan A, Jülicher F. Hydrodynamic flow patterns and synchronization of beating cilia. Physical Review Letters. 2006;96(5):058102.

[14] Niedermayer T, Eckhardt B, Lenz P. Synchronization, phase locking, and metachronal wave formation in ciliary chains. Chaos: An Interdisciplinary Journal of Nonlinear Science. 2008;18(3):0370128.

[15] Vilfan M, Potočnik A, Kavčič B, Osterman N, Poberaj I, Vilfan A, et al. Self-assembled artificial cilia. Proceedings of the National Academy of Sciences. 2010;107(5):1844–1847.

[16] Uchida N, Golestanian R. Synchronization and collective dynamics in a carpet of microfluidic rotors. Physical Review Letters. 2010;104(17):178103.

[17] Uchida N, Golestanian R. Generic conditions for hydrodynamic synchronization. Physical Review Letters. 2011;106(5):058104.

[18] Uchida N, Golestanian R. Hydrodynamic synchronization between objects with cyclic rigid trajectories. The European Physical Journal E, Soft matter. 2012;35(12):9813–9813.

[19] Wollin C, Stark H. Metachronal waves in a chain of rowers with hydrodynamic interactions. The European Physical Journal E. 2011;34(4):1–10.

[20] Guo H, Fauci L, Shelley MJ, Kanso E. Bistability in the synchronization of actuated microfilaments. Journal of Fluid Mechanics. 2018;836:304–323.

[21] Hamilton E, Cicuta P. Changes in geometrical aspects of a simple model of cilia synchronization control the dynamical state, a possible mechanism for switching of swimming gaits in microswimmers. PLOS One. 2021;16(4):e0249060.

[22] Eloy C, Lauga E. Kinematics of the most efficient cilium. Physical Review Letters. 2012 Jul;109(3):038101.

[23] Osterman N, Vilfan A. Finding the ciliary beating pattern with optimal efficiency. Proceedings of the National Academy of Sciences. 2011;108(38):15727–15732.

[24] Kim S, Karrila SJ. Microhydrodynamics: principles and selected applications. Butterworth-Heinemann, Boston, MA; 1991.

[25] Leal LG. Advanced transport phenomena: fluid mechanics and convective transport processes. vol. 7. Cambridge University Press; 2007.

[26] Bird R, Stewart W, Lightfoot E. Transport Phenomena. John Wiley & Sons, Inc; 2007.

[27] Liron N. Fluid transport by cilia between parallel plates. Journal of Fluid Mechanics. 1978;86(04):705–726.

[28] Smith DJ, Gaffney EA, Blake JR. Modelling mucociliary clearance. Respiratory Physiology & Neurobiology. 2008;163(1):178–188.

[29] Guirao B, Joanny JF. Spontaneous creation of macroscopic flow and metachronal waves in an array of cilia. Biophysical Journal. 2007 Mar;92(6):1900–1917.

[30] Ding Y, Nawroth JC, McFall-Ngai MJ, Kanso E. Mixing and transport by ciliary carpets: a numerical study. Journal of Fluid Mechanics. 2014;743:124–140.

[31] Taylor G. Analysis of the swimming of microscopic organisms. Proceedings of the Royal Society of London Series A. 1951;209(1099):447–461.

[32] Pak OS, Lauga E. The transient swimming of a waving sheet. Proceedings of the Royal Society A: Mathematical, Physical and Engineering Sciences. 2010;466(2113):107–126.

[33] Kuramoto Y. Chemical oscillations, waves, and turbulence. Courier Corporation; 2003.

[34] Helgason S, Helgason S. The Radon Transform. Springer; 1980.

[35] Fürthauer S, Ramaswamy S. Phase-Synchronized State of Oriented Active Fluids. Physical Review Letters. 2013 Dec;111:238102.

[36] Ramirez-San Juan GR, Mathijssen AJ, He M, Jan L, Marshall W, Prakash M. Multi-scale spatial heterogeneity enhances particle clearance in airway ciliary arrays. Nature Physics. 2020;16(9):1–7.

[37] Brumley DR, Wan KY, Polin M, Goldstein RE. Flagellar synchronization through direct hydrodynamic interactions. eLife. 2014;3:e02750.

**Algorithm 1** Building the velocity look-up table

**Input:** $n_s$: number of shells
**Input:** $n_\theta$: number of discrete angular points
**Input:** $F(\theta)$: Driving force
**Output:** $T$: Velocity table

Initialize $T$ to a zero matrix of size $(n_\theta N_s, n_\theta, 2)$.
**for** $q = 1 : n_\theta$ **do**
    $\theta^q$: discretized angular location along the circular trajectory
    **for** each rotor inside the stencil $j$ **do**
        $\mathbf{r}_j^q = \mathbf{x}_j + b(\cos\theta^q, \sin\theta^q)$: position vector of each angular location.

**for** each rotor inside the stencil $j$ **do**
    **if** $j \neq i$ **then**
        **for** $q = 1 : n_\theta$ **do**
            Calculate stokeslet strength $\mathbf{F}_j^q$.
            **for** $p = 1 : n_\theta$ **do**
                Compute induced velocity $\mathbf{v}_{i\leftarrow j}^{p,q} = \mathbf{B}(\mathbf{r}_i^p - \mathbf{r}_j^q) \cdot \mathbf{F}_j^q$
                Append $\mathbf{v}_{i\leftarrow j}^{p,q}$ to table $T$

**Algorithm 2** Computing induced velocities using look-up

**Input:** $\theta_i$,: angular phase of the $i$-th cilium
**Input:** $\mathcal{N}(i)$: list of interacting neighbors for $i$-th cilium $i$
**Input:** Velocity table $T$
**Output:** $\mathbf{v}_i$: Induced velocity on $i$-th cilium

Using $\theta_i$, find the two nearest angular grid points $\theta_i^p$, $\theta_i^{p+1}$
**for all** $j \in \mathcal{N}(i)$ **do**
    Using $\theta_j$, find the two nearest angular grid points $\theta_j^q$, $\theta_j^{q+1}$
    look-up $\mathbf{v}_{i\leftarrow j}^{p,q}$, $\mathbf{v}_{i\leftarrow j}^{p,q+1}$, $\mathbf{v}_{i\leftarrow j}^{p+1,q}$, $\mathbf{v}_{i\leftarrow j}^{p+1,q+1}$
    Use bi-linear interpolation to evaluate $\mathbf{v}_{i\leftarrow j}$

$\mathbf{v}_i = \sum_{j\in\mathcal{N}(i)} \mathbf{v}_{i\leftarrow j}$: total velocity induced on cilium $i$

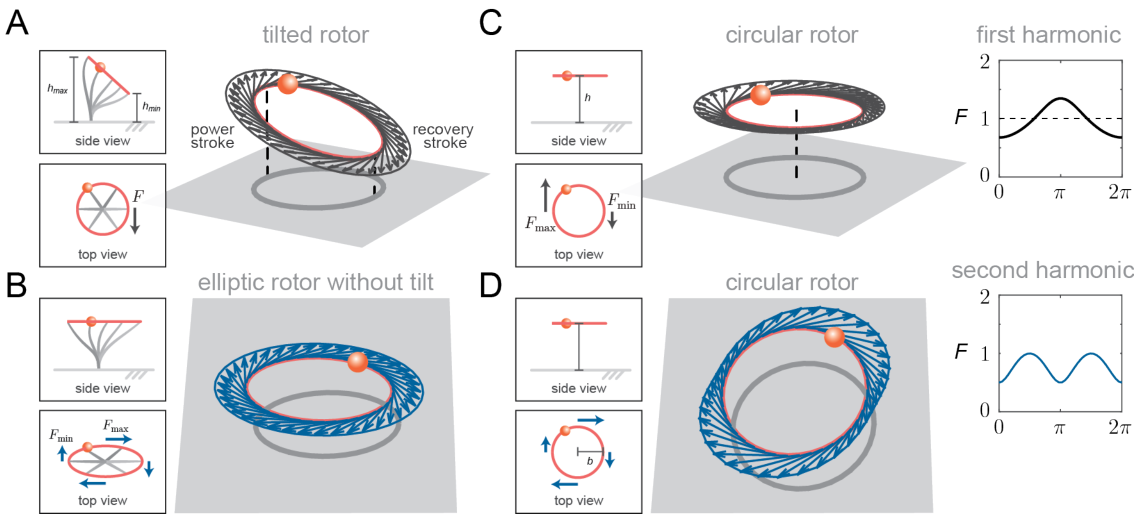


Figure S.1: **Cilia as circular phased oscillators.** (A) Asymmetric power and recovery strokes are captured by a tilted rotor traveling with constant angular velocity [23, 37]. (B) Cilia that beat with no preferred direction can be effectively modeled as a rotor of constant angular velocity that follows an elliptic trajectory. (C) The far-field flow due to the tilted rotor can be modeled by the first harmonic forcing perturbation. (D) Similarly, the far-field flow effects of a rotor following an elliptical trajectory can be captured by a circular rotor following a second harmonic forcing perturbation. Nonlinear least-squares fitting is used to optimize $F(\theta)$ by minimizing the difference in the flow fields between (A) and (C) and between (B) and (D) on a set of $20 \times 20 \times 20$ grid points $\boldsymbol{p}$ spaced evenly in the zone $[-4b, 4b] \times [-4b, 4b] \times [0.1h, 40h]$.

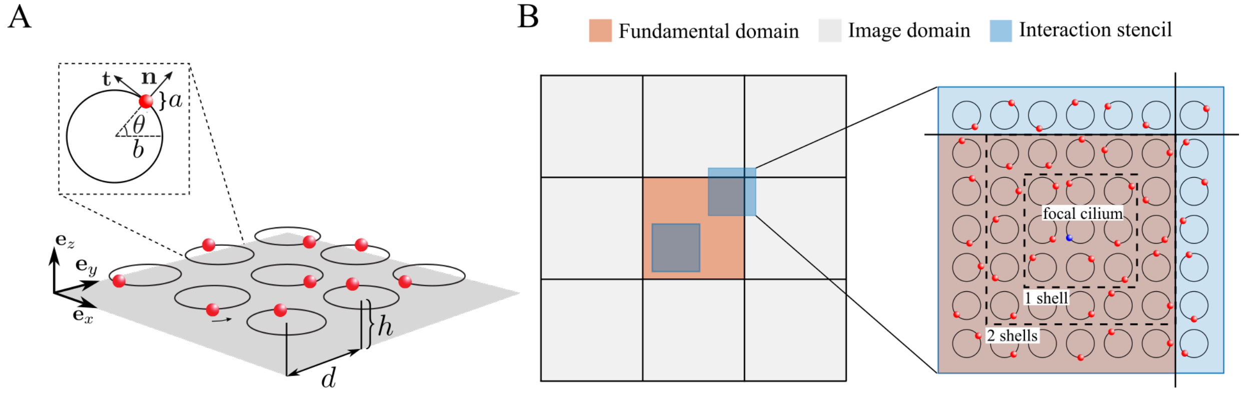


Figure S.2: **Ciliary Layer:** (A) a doubly-infinite lattice of cilia, where each cilium modeled as a bead rotating on a fixed circular trajectory under the influence of a positive phase-dependent force $F(\theta)$. Cilia are arranged on a square lattice, with lattice spacing $d$, at a distance $h$ above a no-slip boundary. (B) The computational domain, consisting of the fundamental domain (red), images (gray) and interaction stencil (blue). Zooming-in on the interaction stencil shows the focal cilium at the center of the lattice (dark blue) and the neighboring cilia (red).

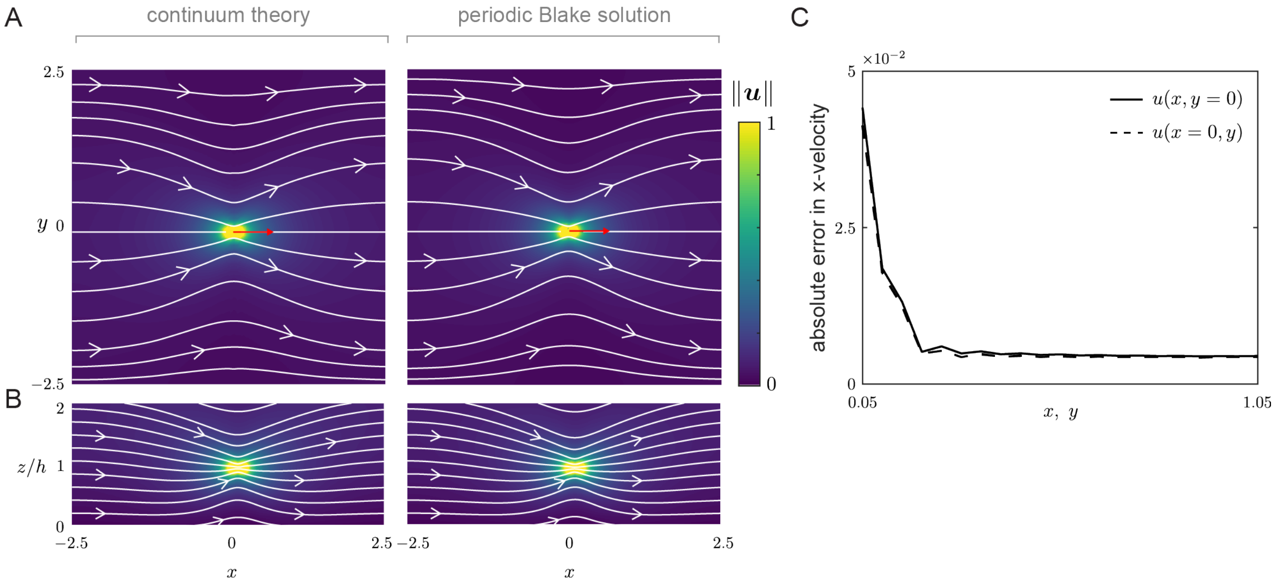


Figure S.3: Comparison of flow fields created by a unit force monopole in the 3D half-space, oriented in the positive $x$-direction. (A) Flow fields in the ciliary plane and (B) Flow fields in a plane perpendicular to the ciliary plane based on the continuum theory (left) and Blake-Oseen solution (right). Velocity magnitude $\|\mathbf{u}\|$ is shown as a colormap and streamlines in white lines. To emulate the effect of a doubly-periodic lattice, the fundamental domain is surrounded by five concentric shells of image domains. (C) Absolute value of the difference in the $x$-component of the velocity $u(x, y, z = h)$ along $y = 0$ (solid) and $x = 0$ (dashed) at $z = h$.

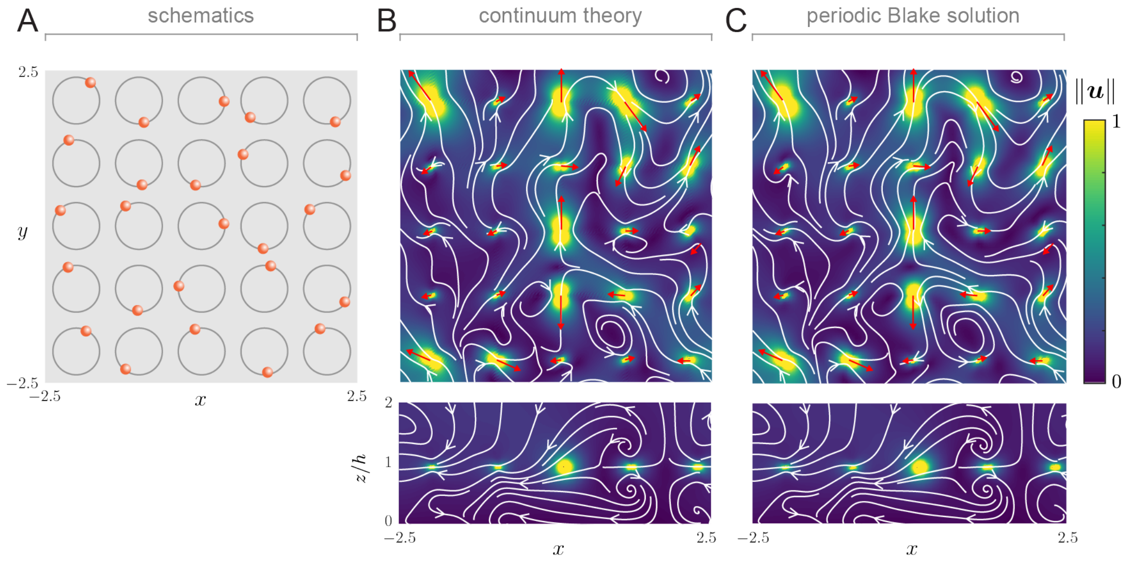


Figure S.4: **Comparison of flow fields created by a lattice of force monopoles in the 3D half-space (random directions).** (A) Schematic depiction of a lattice of cilia at random phase. (B) Flow field in the ciliary plane, flow magnitude (colormap) and streamlines (white lines), based on the continuum theory (left) and particle model (right), respectively. The red arrows indicate the relative strength and orientation of each force monopole. (C) Flow field in a plane perpendicular to the ciliary plane.

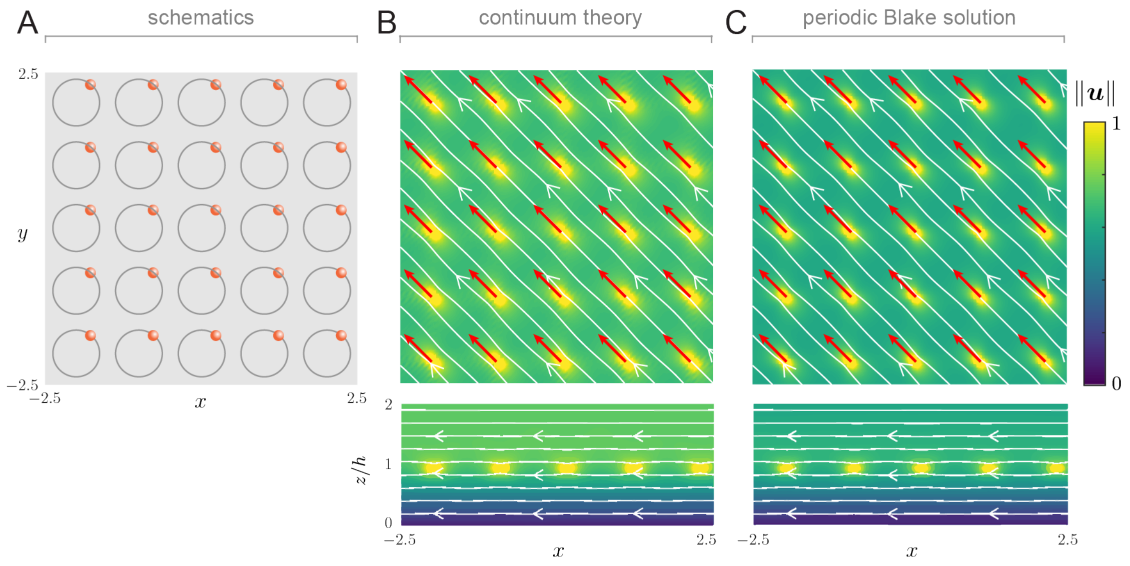


Figure S.5: **Comparison of flow fields created by a lattice of force monopoles in the 3D half-space (uniform directions).** (A) Schematic depiction of a lattice of fully synchronized cilia. (B) Flow field in the ciliary plane, flow magnitude (colormap) and streamlines (white lines), based on the continuum theory (left) and particle model (right), respectively. The red arrows indicate the relative strength and orientation of each stokeslet. (C) Flow field in a plane perpendicular to the ciliary plane.

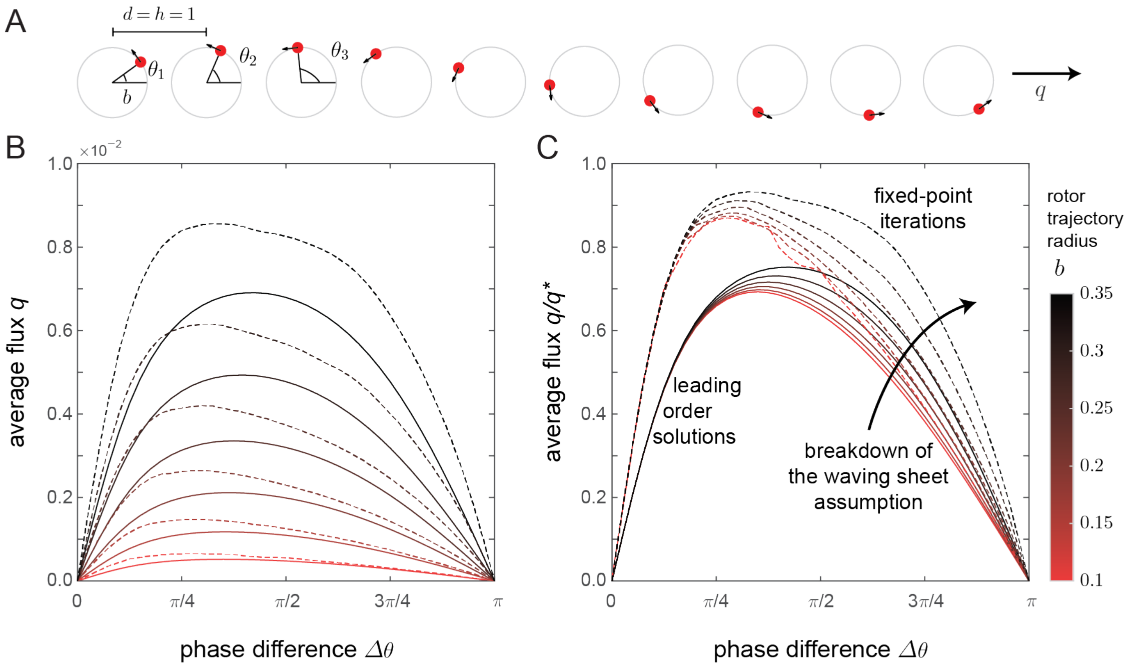


Figure S.6: **Net flux versus phase lag in a 1D array of rotors.** (A) Given a 1D array of $N = 10$ rotors with constant rotating speed $\Omega = 1$ and fixed phase difference $\Delta\theta$, the flux $q$ produced by the metachronal wave is in the opposite direction of rotor rotation (B) $\langle q \rangle$ is computed with $O(\mathbf{B}^2)$ terms ignored (solid lines), or considered via fixed point iterations (dashed lines); see§ S.2.2. (C) When the average qux is scaled by the characteristic fluid pumping scale $q^*$, solution curves collapse for small trajectory radius $b$ and phase difference $\Delta\theta$. This is because in the limit of $b/d \to 0, \Delta\theta \to 0$, the prescribed rotor system can be adequately approximated by a continuous waving sheet *e.g.,* Taylor's swimming sheet and Blake's envelope model [1,31,32]. These results numerically validate both our flux computation and our assumption of ignoring $O(\mathbf{B}^2)$ terms when computing the phase dynamics and emergent coordination in 2D lattices.

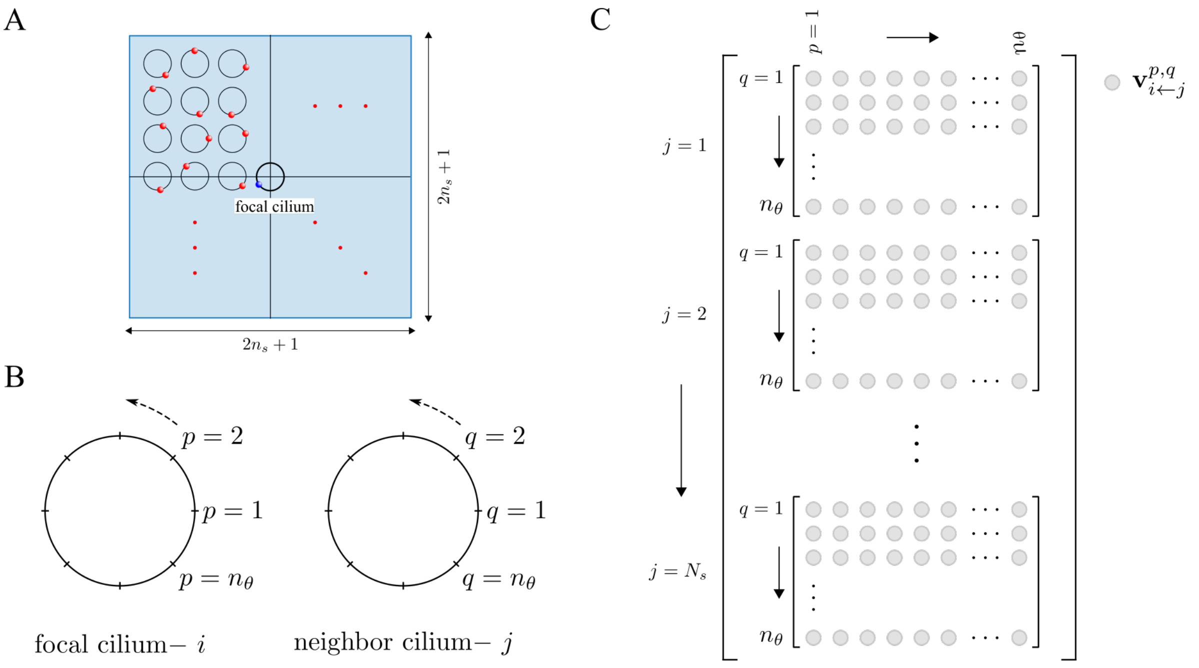


Figure S.7: (A) Induced velocities at the location of the focal cilium (blue), by every other cilium inside the interaction stencil (red) are pre-computed and stored. (B) The trajectory of each cilium is discretized into $n_\theta$ angular locations. $\mathbf{v}_{i\leftarrow j}^{p,q}$ is the induced velocity at angular location $p$ of the focal cilium $i$, due a neighboring cilium, $j$, at angular location $q$, and is computed using the Blake tensor. (C) Schematic representation of the velocity look-up table. Each entry is a 2D velocity vector populated by computed at each pair of locations shown in panel (B).

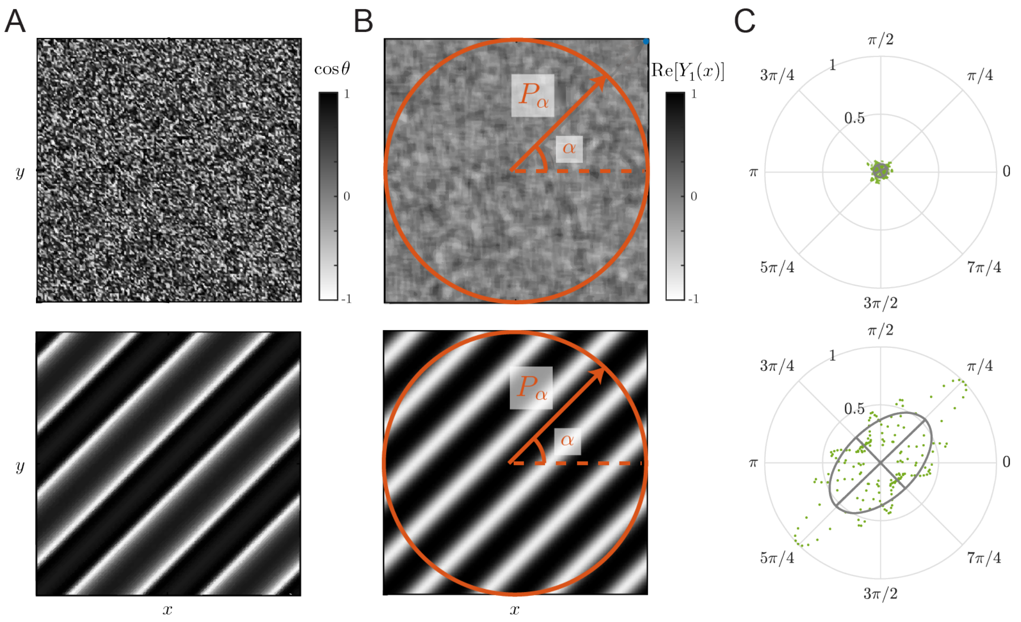


Figure S.8: **Kuramoto Ellipse.** Using snapshots of an isotropic state (top) and a synthetically created wave state (bottom) to illustrate the usage of Kuramoto ellipse. **A.** The cosine field, obtained by taking the cosine of the phase of the cilium. **B.** The corresponding Kuramoto order field– Real($Y_1(\mathbf{x})$)– which is calculated by coarse graining over one shell of neighbors. **C.** Polar coordinates $(\alpha, P(\alpha))$ in green, and the corresponding Kuramoto ellipse in gray.

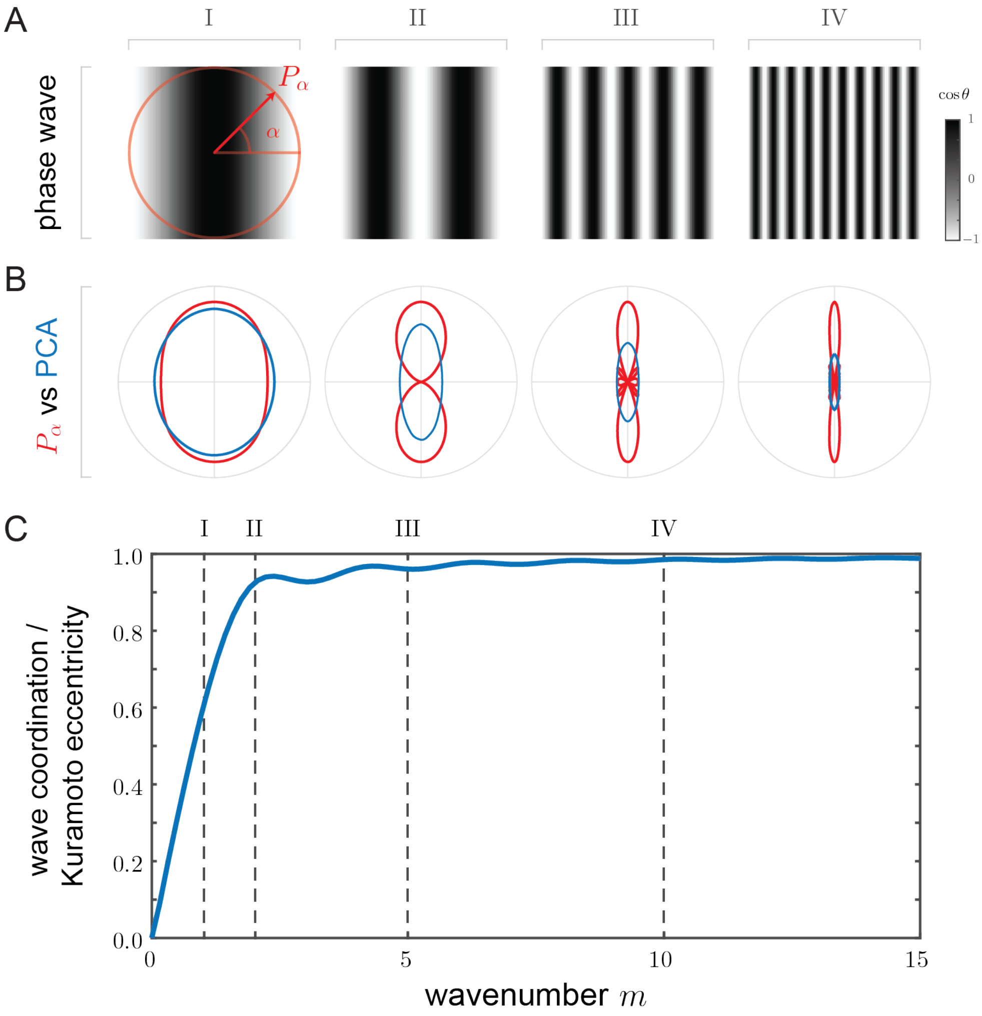


Figure S.9: **Eccentricity of the Kuramoto ellipse.** (A) To probe how the eccentricity of the Kuramoto ellipse depends on the wave characteristics, we calculate the eccentricity using simple phase waves that travel in the horizontal direction, *i.e.*, $\theta = mx/L$. (B) The quantity $P_\alpha = |\int_0^{L/2} Y_1(s\cos\alpha, s\sin\alpha)\,\mathrm{d}s|$ can be computed analytically to be $2|\sec\alpha\sin((m\cos\alpha)/4)|/m$. Performing PCA on $(\alpha, P_\alpha)$ as before, we obtain the blue ellipses. (C) The Kuramoto eccentricity as a function of the wavenumber $m$. In the synchronized state, at wavenumber $m = 0$, there is no wave and the eccentricity is zero. As the wavenumber increases, the eccentricity quickly rise to a value near 1. In the limit of infinite wavenumber, the theoretical eccentricity is 1. However, in discrete numerical computations, wavenumbers greater than those dictated by the rotor distance $\pi/d$ introduce aliasing effects. Note that eccentricity is also zero in the limit of isotropic phase distribution (see Fig. S.8).

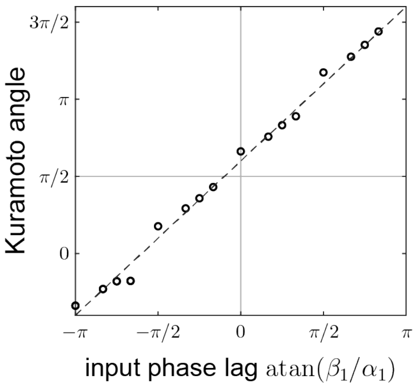


Figure S.10: **Kuramoto angle is orthogonal to the direction of wave propagation.** When subject to a first force harmonic, $F(\theta) = F_o(1 + \alpha_1 \cos\theta + \beta_1 \sin\theta)$, the emergent coordination consists of waves that propagate in the same direction as the direction from minimum to maximum forcing, that is, in the same direction as the phase lag $\arctan(\beta_1/\alpha_1)$. Evidently, the Kuramoto angle is linearly correlated with $\arctan(\beta_1/\alpha_1)$ and is roughly orthogonal. Here, the Kuramoto angle was measured using the steady state from simulation data of a 151 x 151 lattice of cilia for $b = h = 1$, $d = 3$, $F_o = 1$ and $\sqrt{\alpha_1^2 + \beta_1^2} = 0.5$.

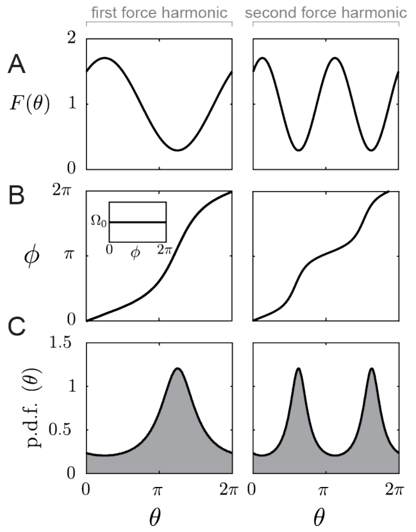


Figure S.11: **Nonlinear phase transformation.** (A) Force profiles, $F(\theta)$, corresponding to the first and second harmonics in (23). (B) the transformation from angular phase $\theta$ to a new phase $\phi$ in which the intrinsic angular speed, $\Omega_0 = 2\pi/T_0$, of a single cilium is constant (shown in inset). Here, $T_0$ is the intrinsic time period defined by $\int_0^{2\pi} d\bar{\theta}/\Omega(\bar{\theta})$ and is invariant with the force harmonic, since the integrals of the sine and cosine terms drop out. (C) Cilia that are uniformly distributed in $\phi$ ($\phi \in \mathrm{Unif}[0, 2\pi)$) exhibit a non-uniform distribution in $\theta$ that reflect main features of the force harmonic: single-peak distribution for the first force harmonic, double-peak distribution for the second force harmonic, and so on.

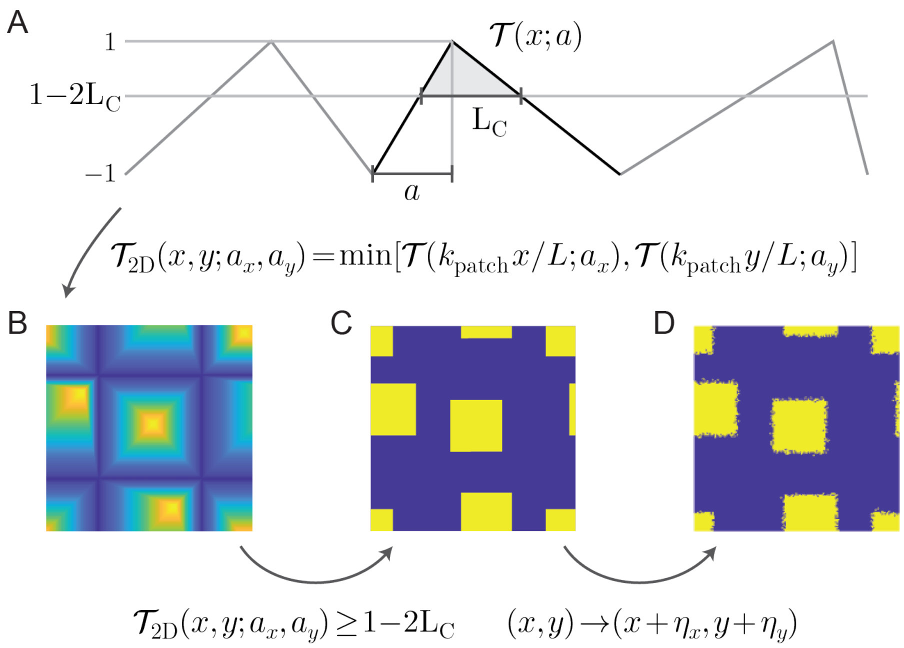


Figure S.12: **Heterogeneous organization of cilia.** (A) We start from a 1D triangular wave function and allow the location $a$ of the peaks within each wavelength to be arbitrary. (B) We re-parameterize two such functions and combine them using the minimum function to arrive at a color map over the cilia fundamental domain. (C) We transform this colormap into a binary function by ignoring all values below a given threshold (blue region) and setting to a constant all values above that threshold (yellow regions). Applying the threshold at $1-2L_C$ returns an area coverage fraction of $C = L_C^2$. (D) Rotor displacement noise can be added via a further re-parameterization.
